# Supplementary material for: International vulnerability of inflation
Source: arXiv:2410.20628 source file (2024-10-29)
Supplement: Supplementary file 1 [file Appendix.tex]

\newpage

\onehalfspacing

\begin{center}
\section*{\large{Online Appendix\\International vulnerability of inflation}}
\end{center}

\addcontentsline{toc}{section}{Supplementary material}

\vspace{0.5cm}

\subsection{Results of  out-of-sample rolling-window estimation.}

We consider first the factors extracted in each estimation sample of the rolling window. Figure \ref{fig:vintage_factors} plots the estimates of each of the factors obtained in each rolling-window period. This figure shows that the factors extracted are rather consistent through vintages. 
   
\begin{figure}[]
\caption{Vintages of factors extracted in each estimation period in the rolling-window.}
\label{fig:vintage_factors}
\begin{center}
\subfigure[Global factor]{\includegraphics[width=0.4\textwidth]{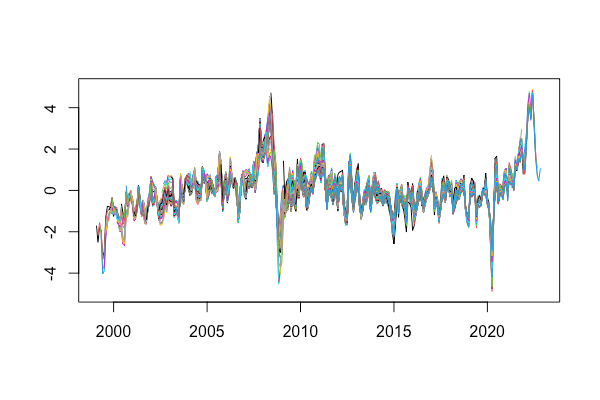}}\\
\subfigure[African factor]{\includegraphics[width=0.4\textwidth]{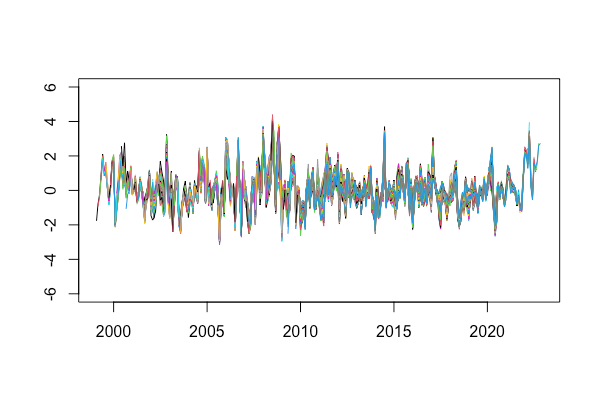}}
\subfigure[Advanced economies factor]{\includegraphics[width=0.4\textwidth]{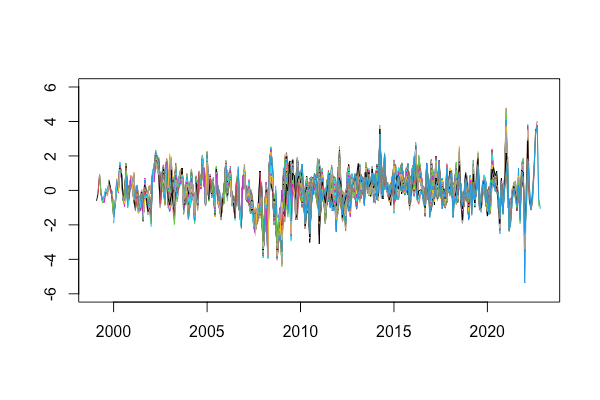}}
\subfigure[American factor]{\includegraphics[width=0.4\textwidth]{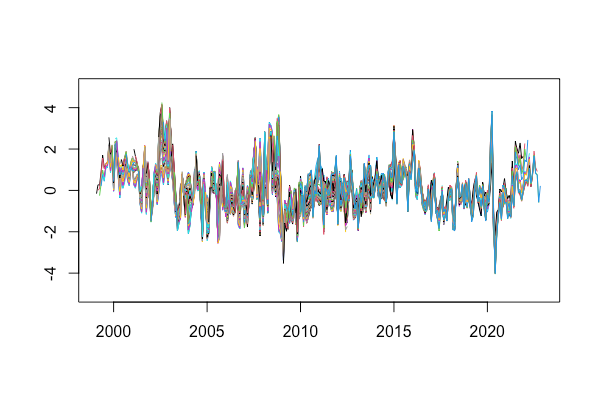}}
\subfigure[HMI economies factor]{\includegraphics[width=0.4\textwidth]{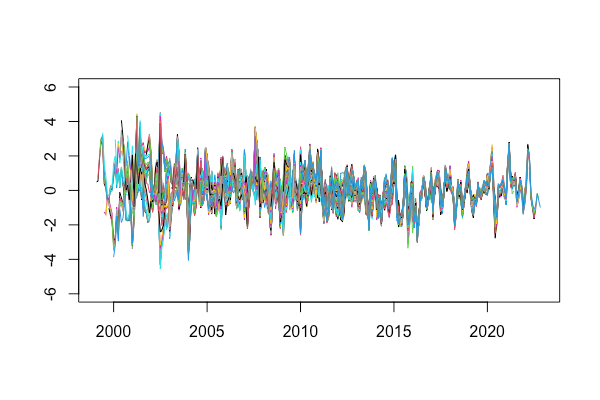}}
\subfigure[Asian factor]{\includegraphics[width=0.4\textwidth]{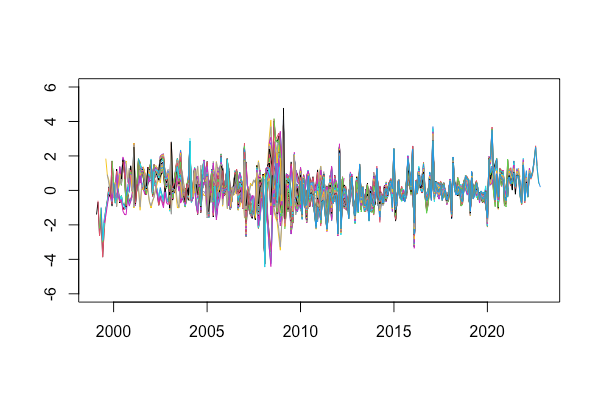}}
\subfigure[LI economies factor]{\includegraphics[width=0.4\textwidth]{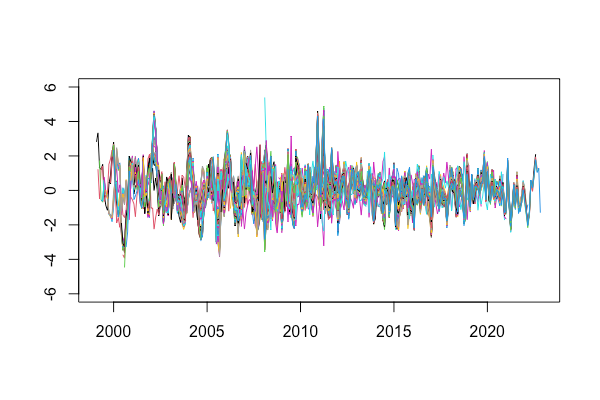}}
\end{center}
\subfigure[European factor]{\includegraphics[width=0.40\textwidth]{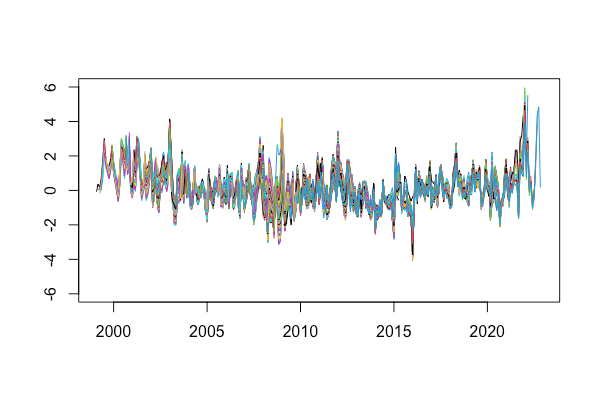}}
\end{figure}

We also consider the possibility of time-varying parameters of the FA-QR model. Figure \ref{fig:tv_estimates} plots the estimated parameters of each quantile obtained in each rolling-window vintage for Italy, the US and Mexico. It is remarkable to see that the parameter associated to the global factor is increasing through time for the upper 95\% quantile in the US and Mexico, but for the very last years associated to the Ukraine invasion. Furthermore, the parameter associated to the regional factor is increasing through time in Italy and decreasing in Mexico. Finally, it is also important to note the increasing parameter of the factor related with the level of economic development in the 50\%, 75\% and 95\% quantiles in Mexico.

\begin{figure}[]
\begin{center}
\subfigure[]{\includegraphics[width=0.30\textwidth]{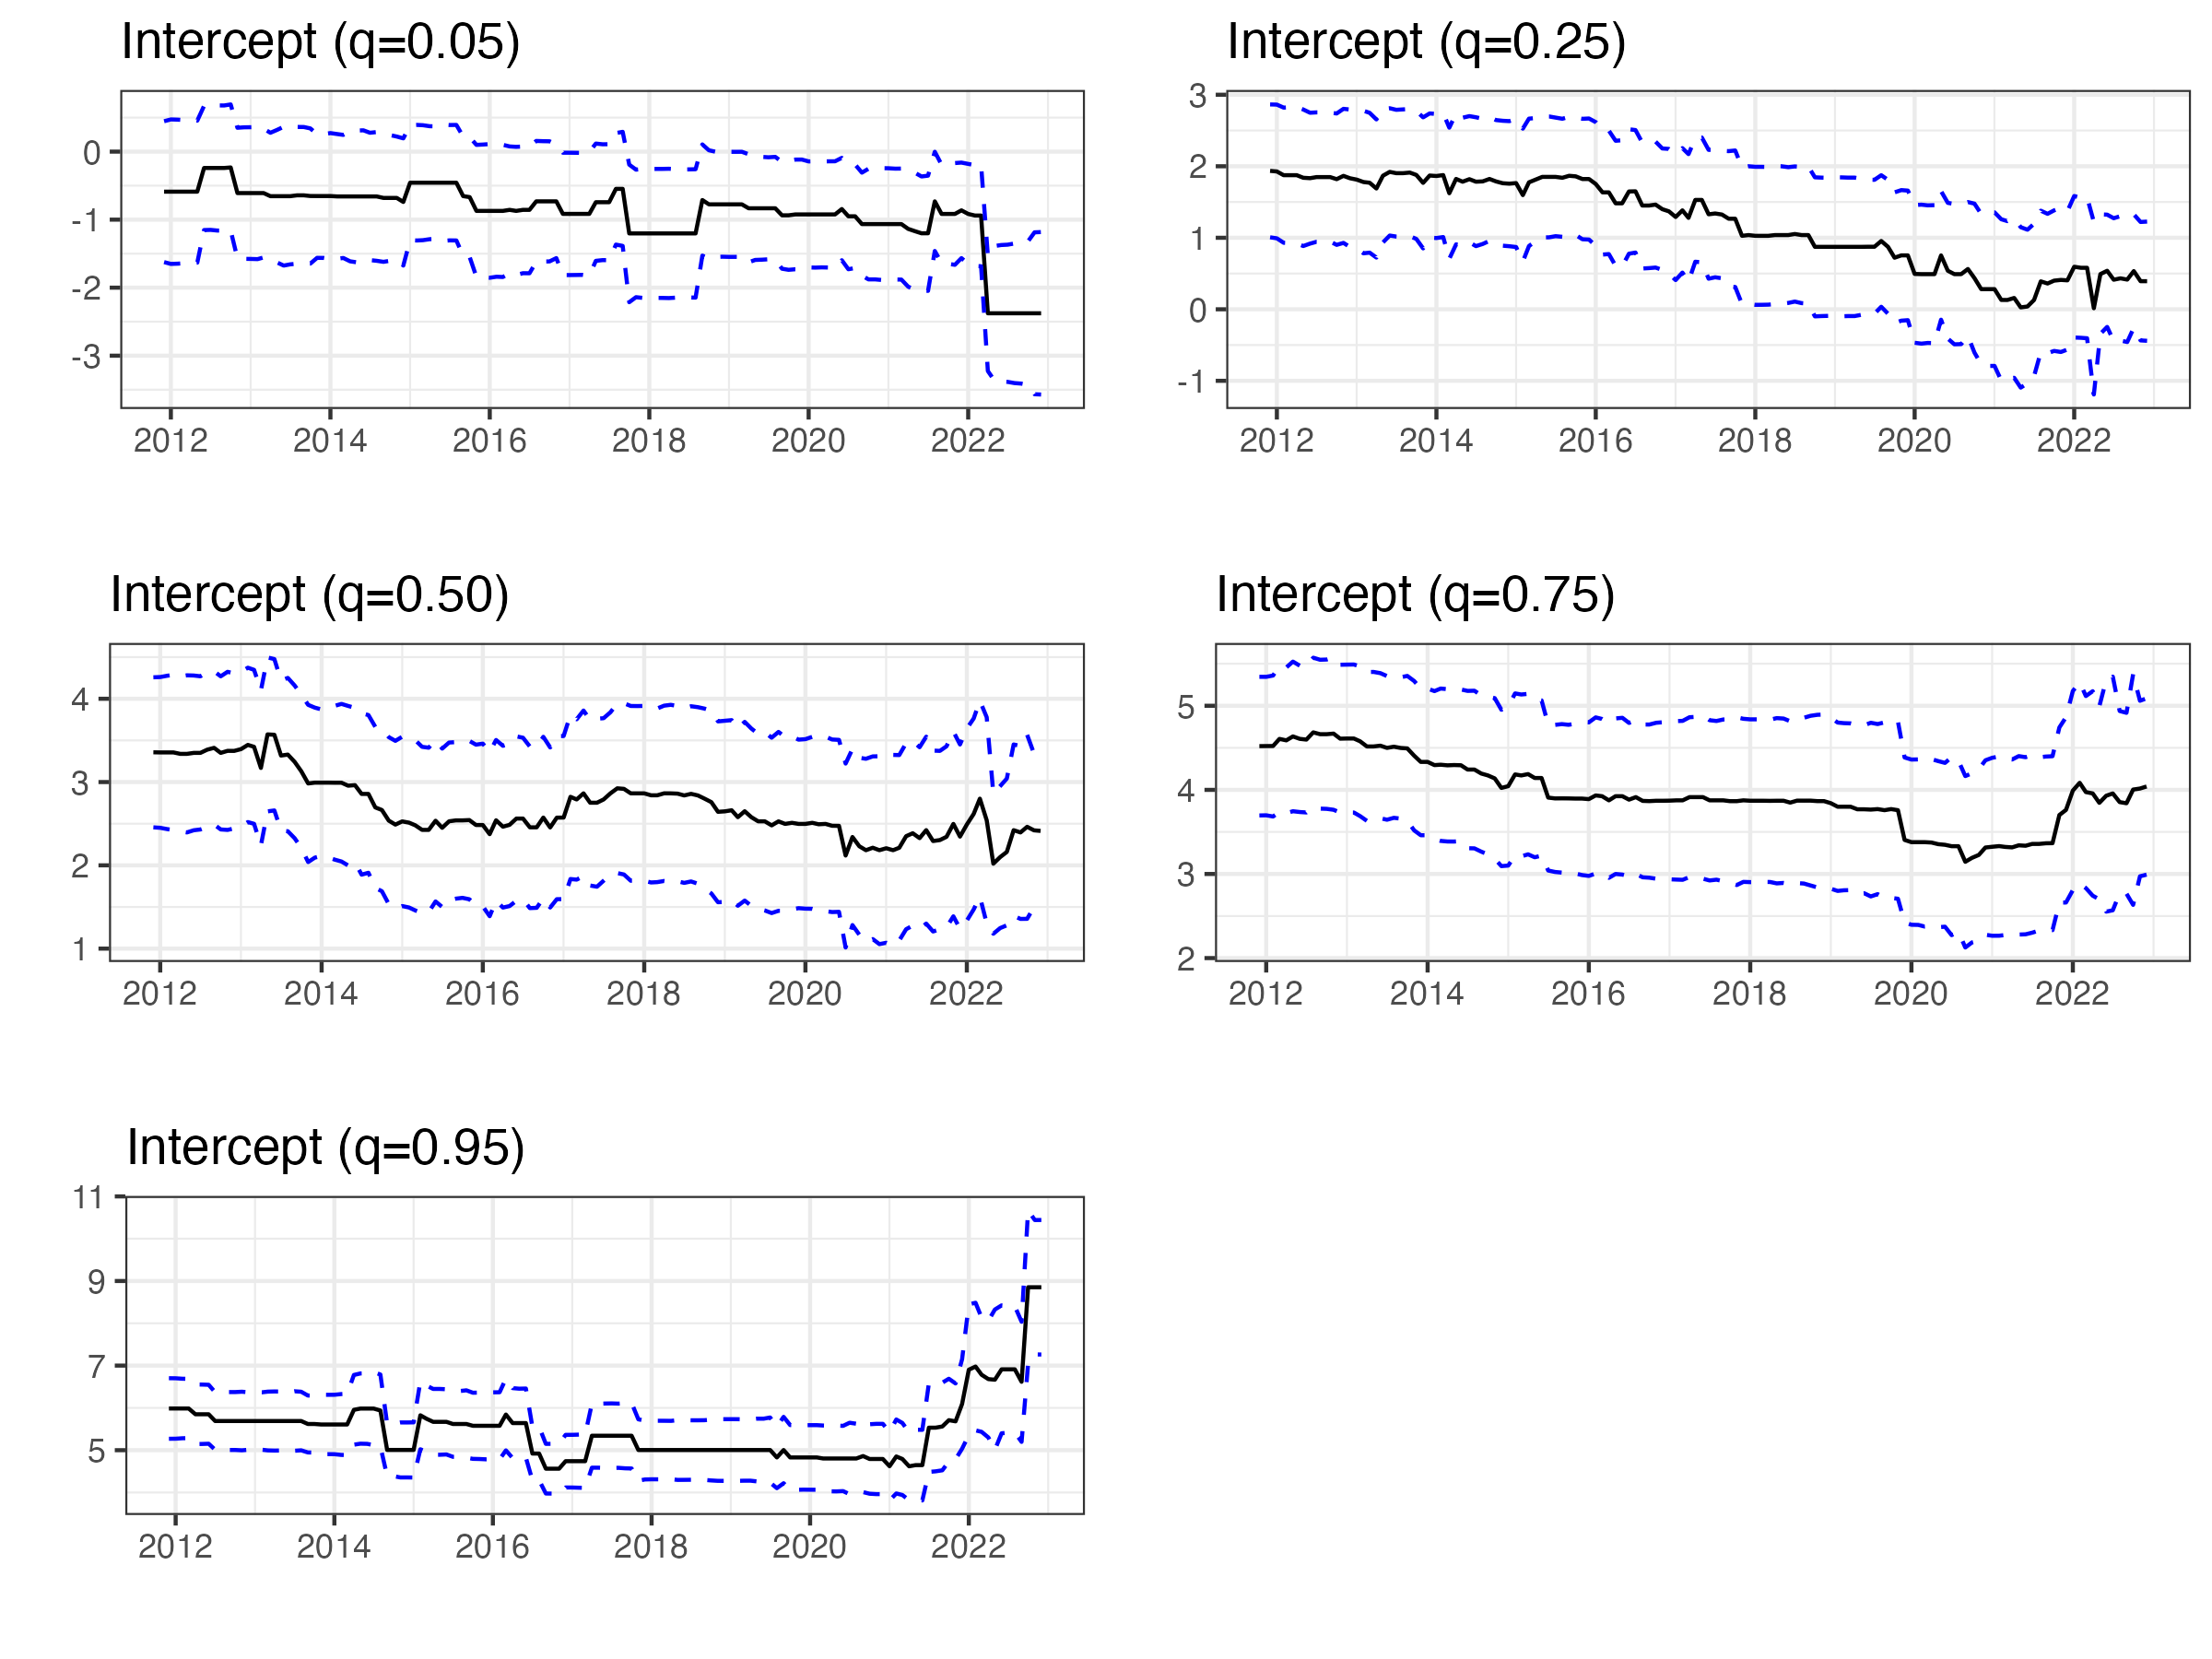}}
\subfigure[]{\includegraphics[width=0.30\textwidth]{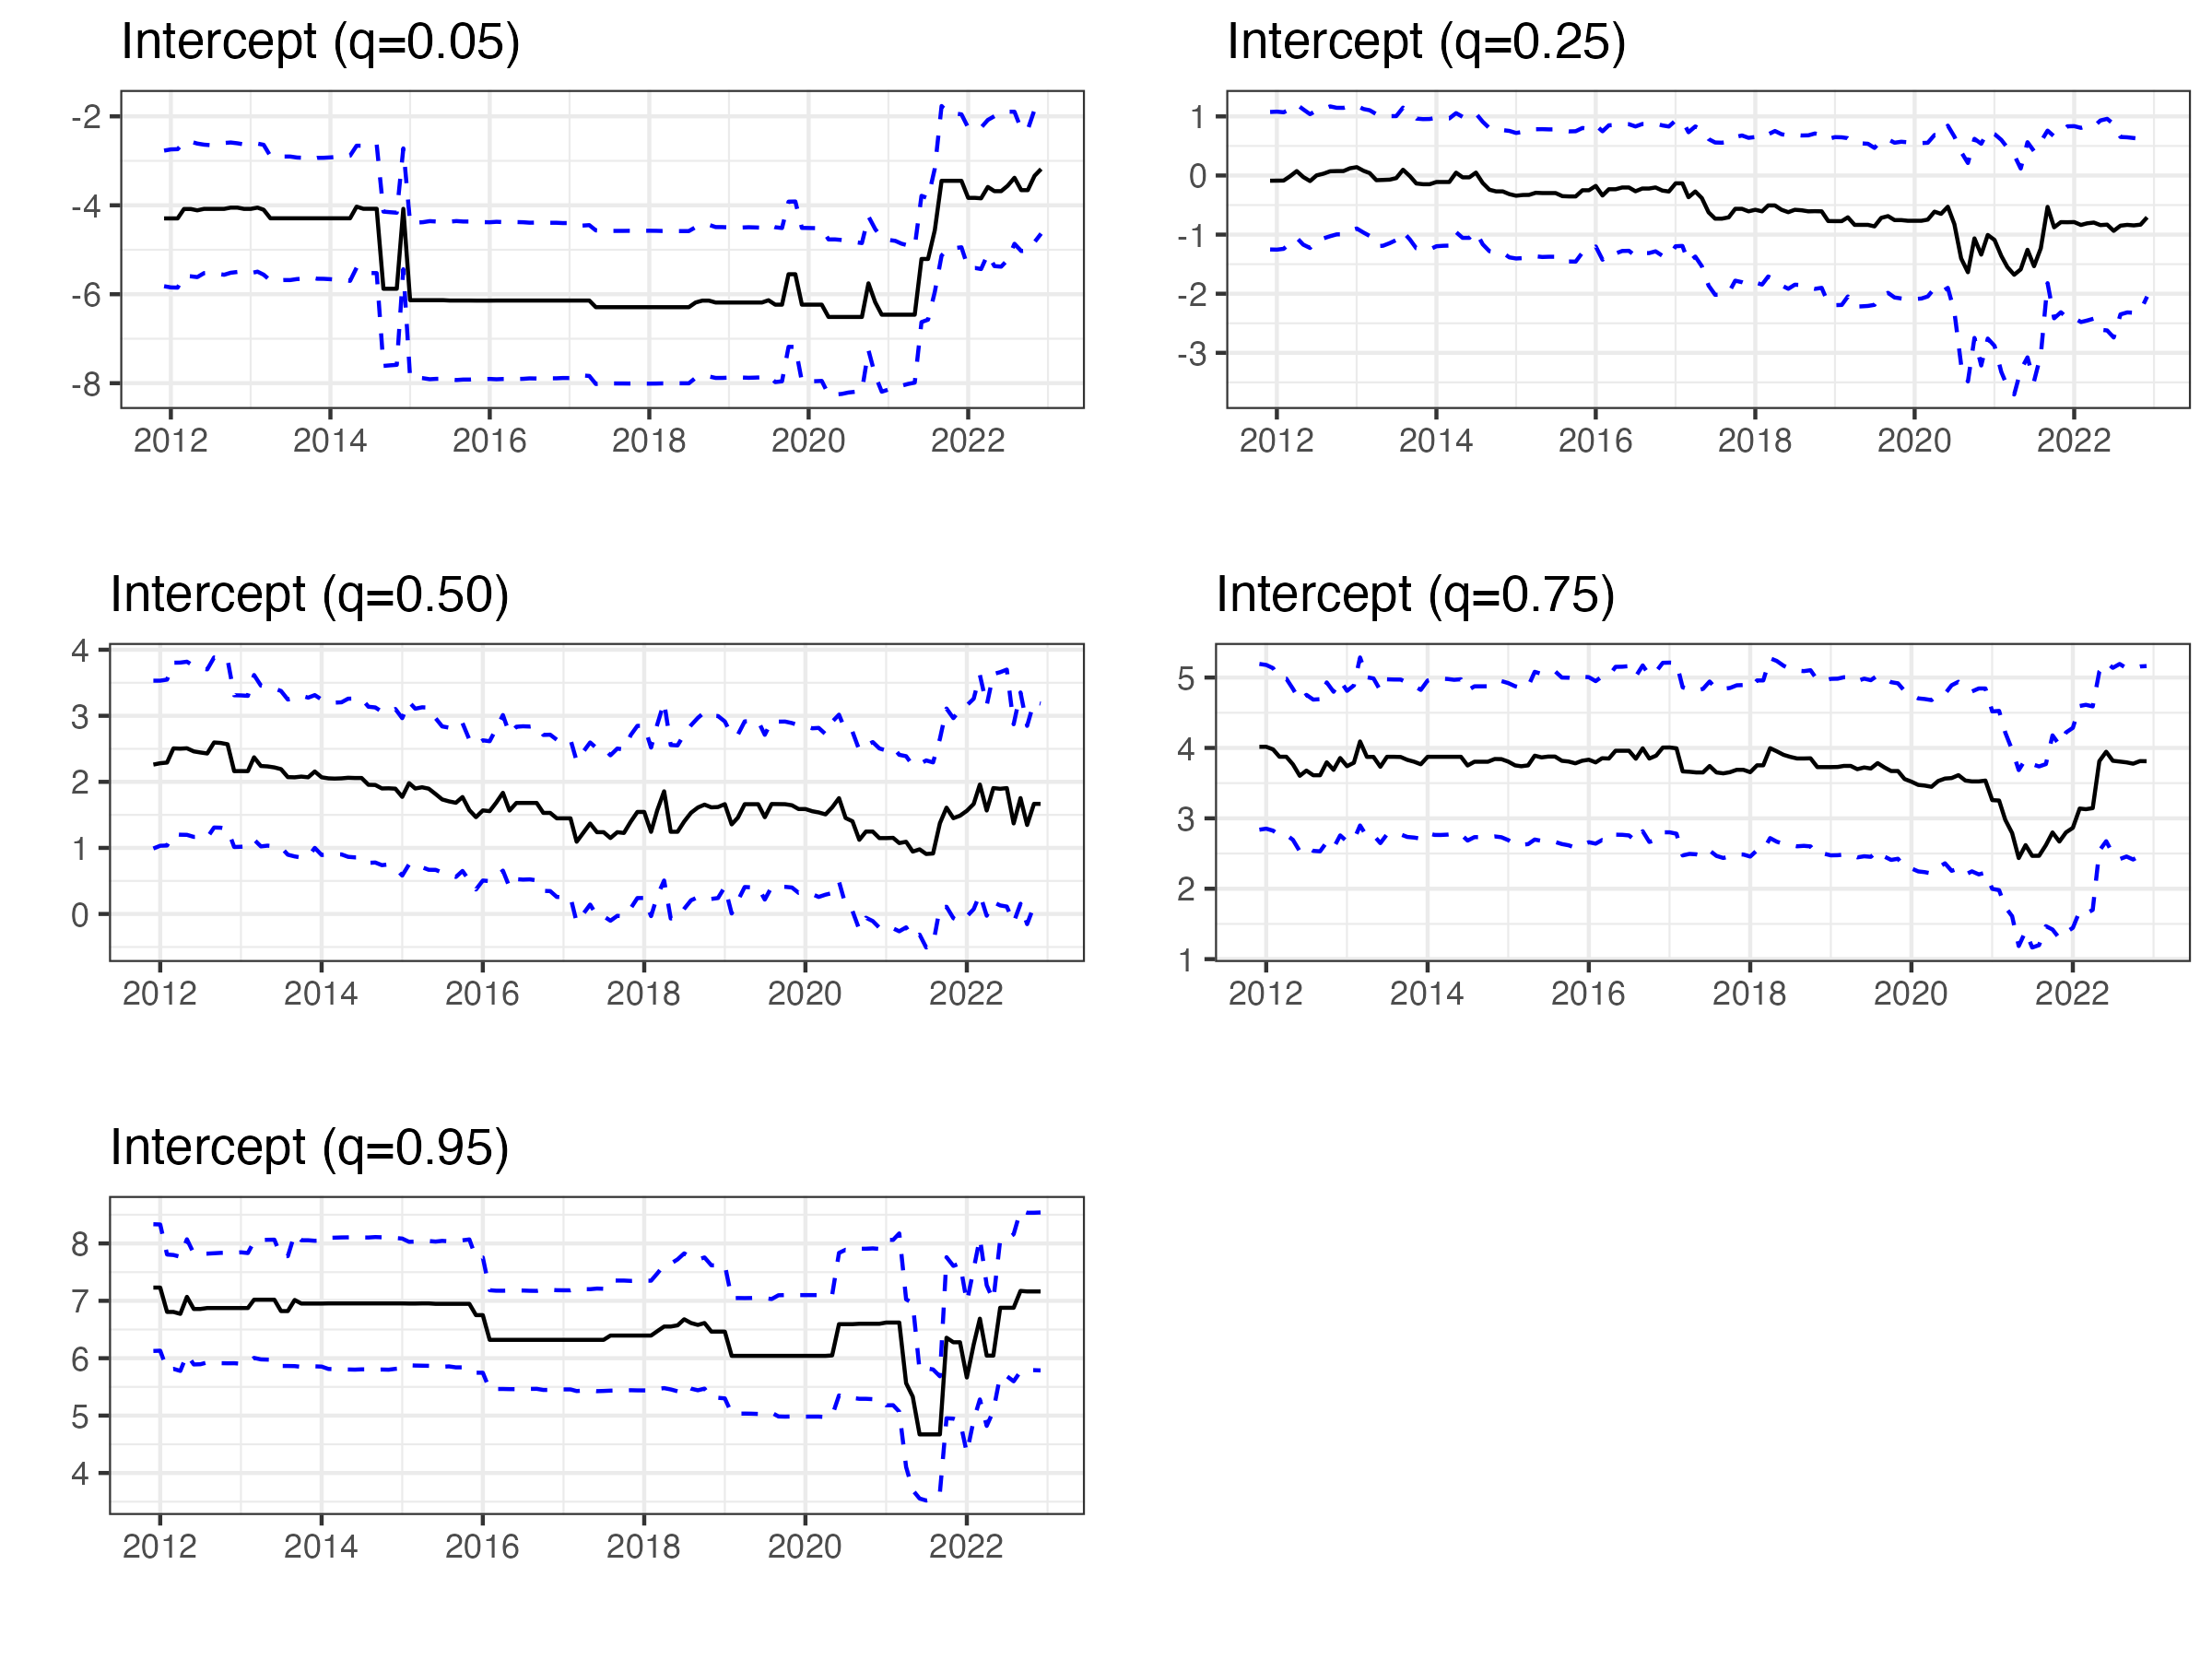}}
\subfigure[]{\includegraphics[width=0.30\textwidth]{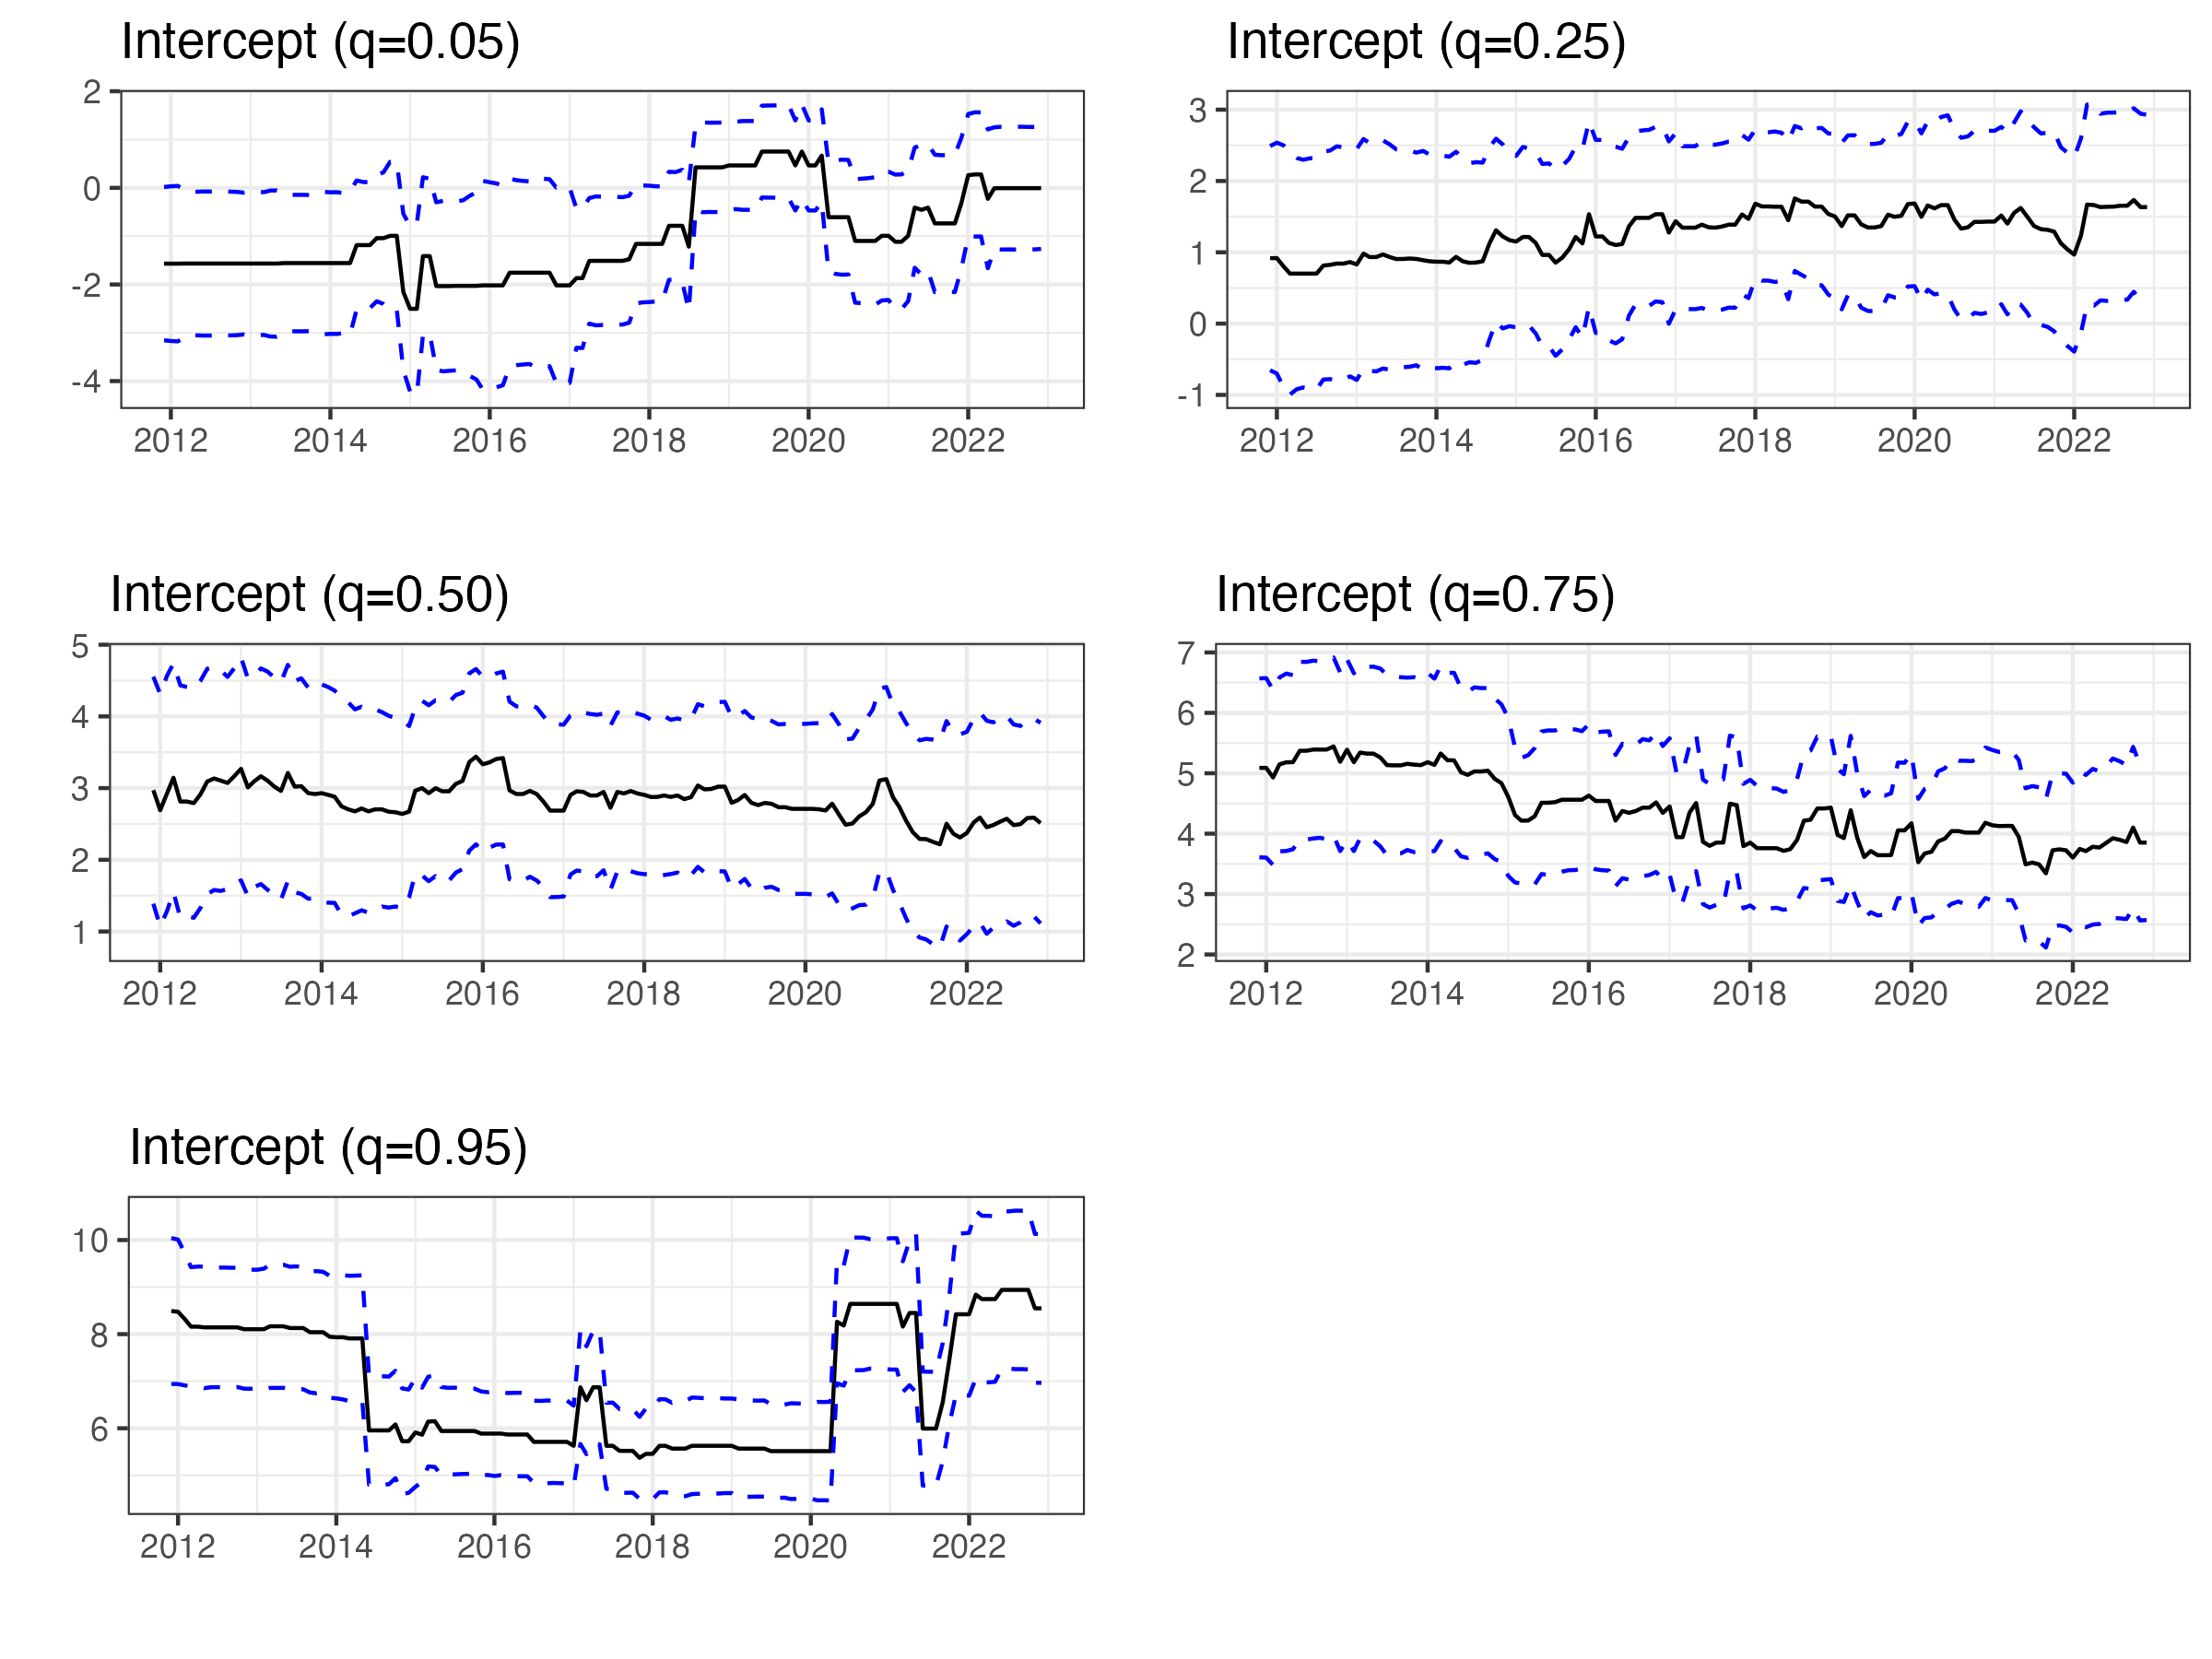}}\\
\subfigure[]{\includegraphics[width=0.30\textwidth]{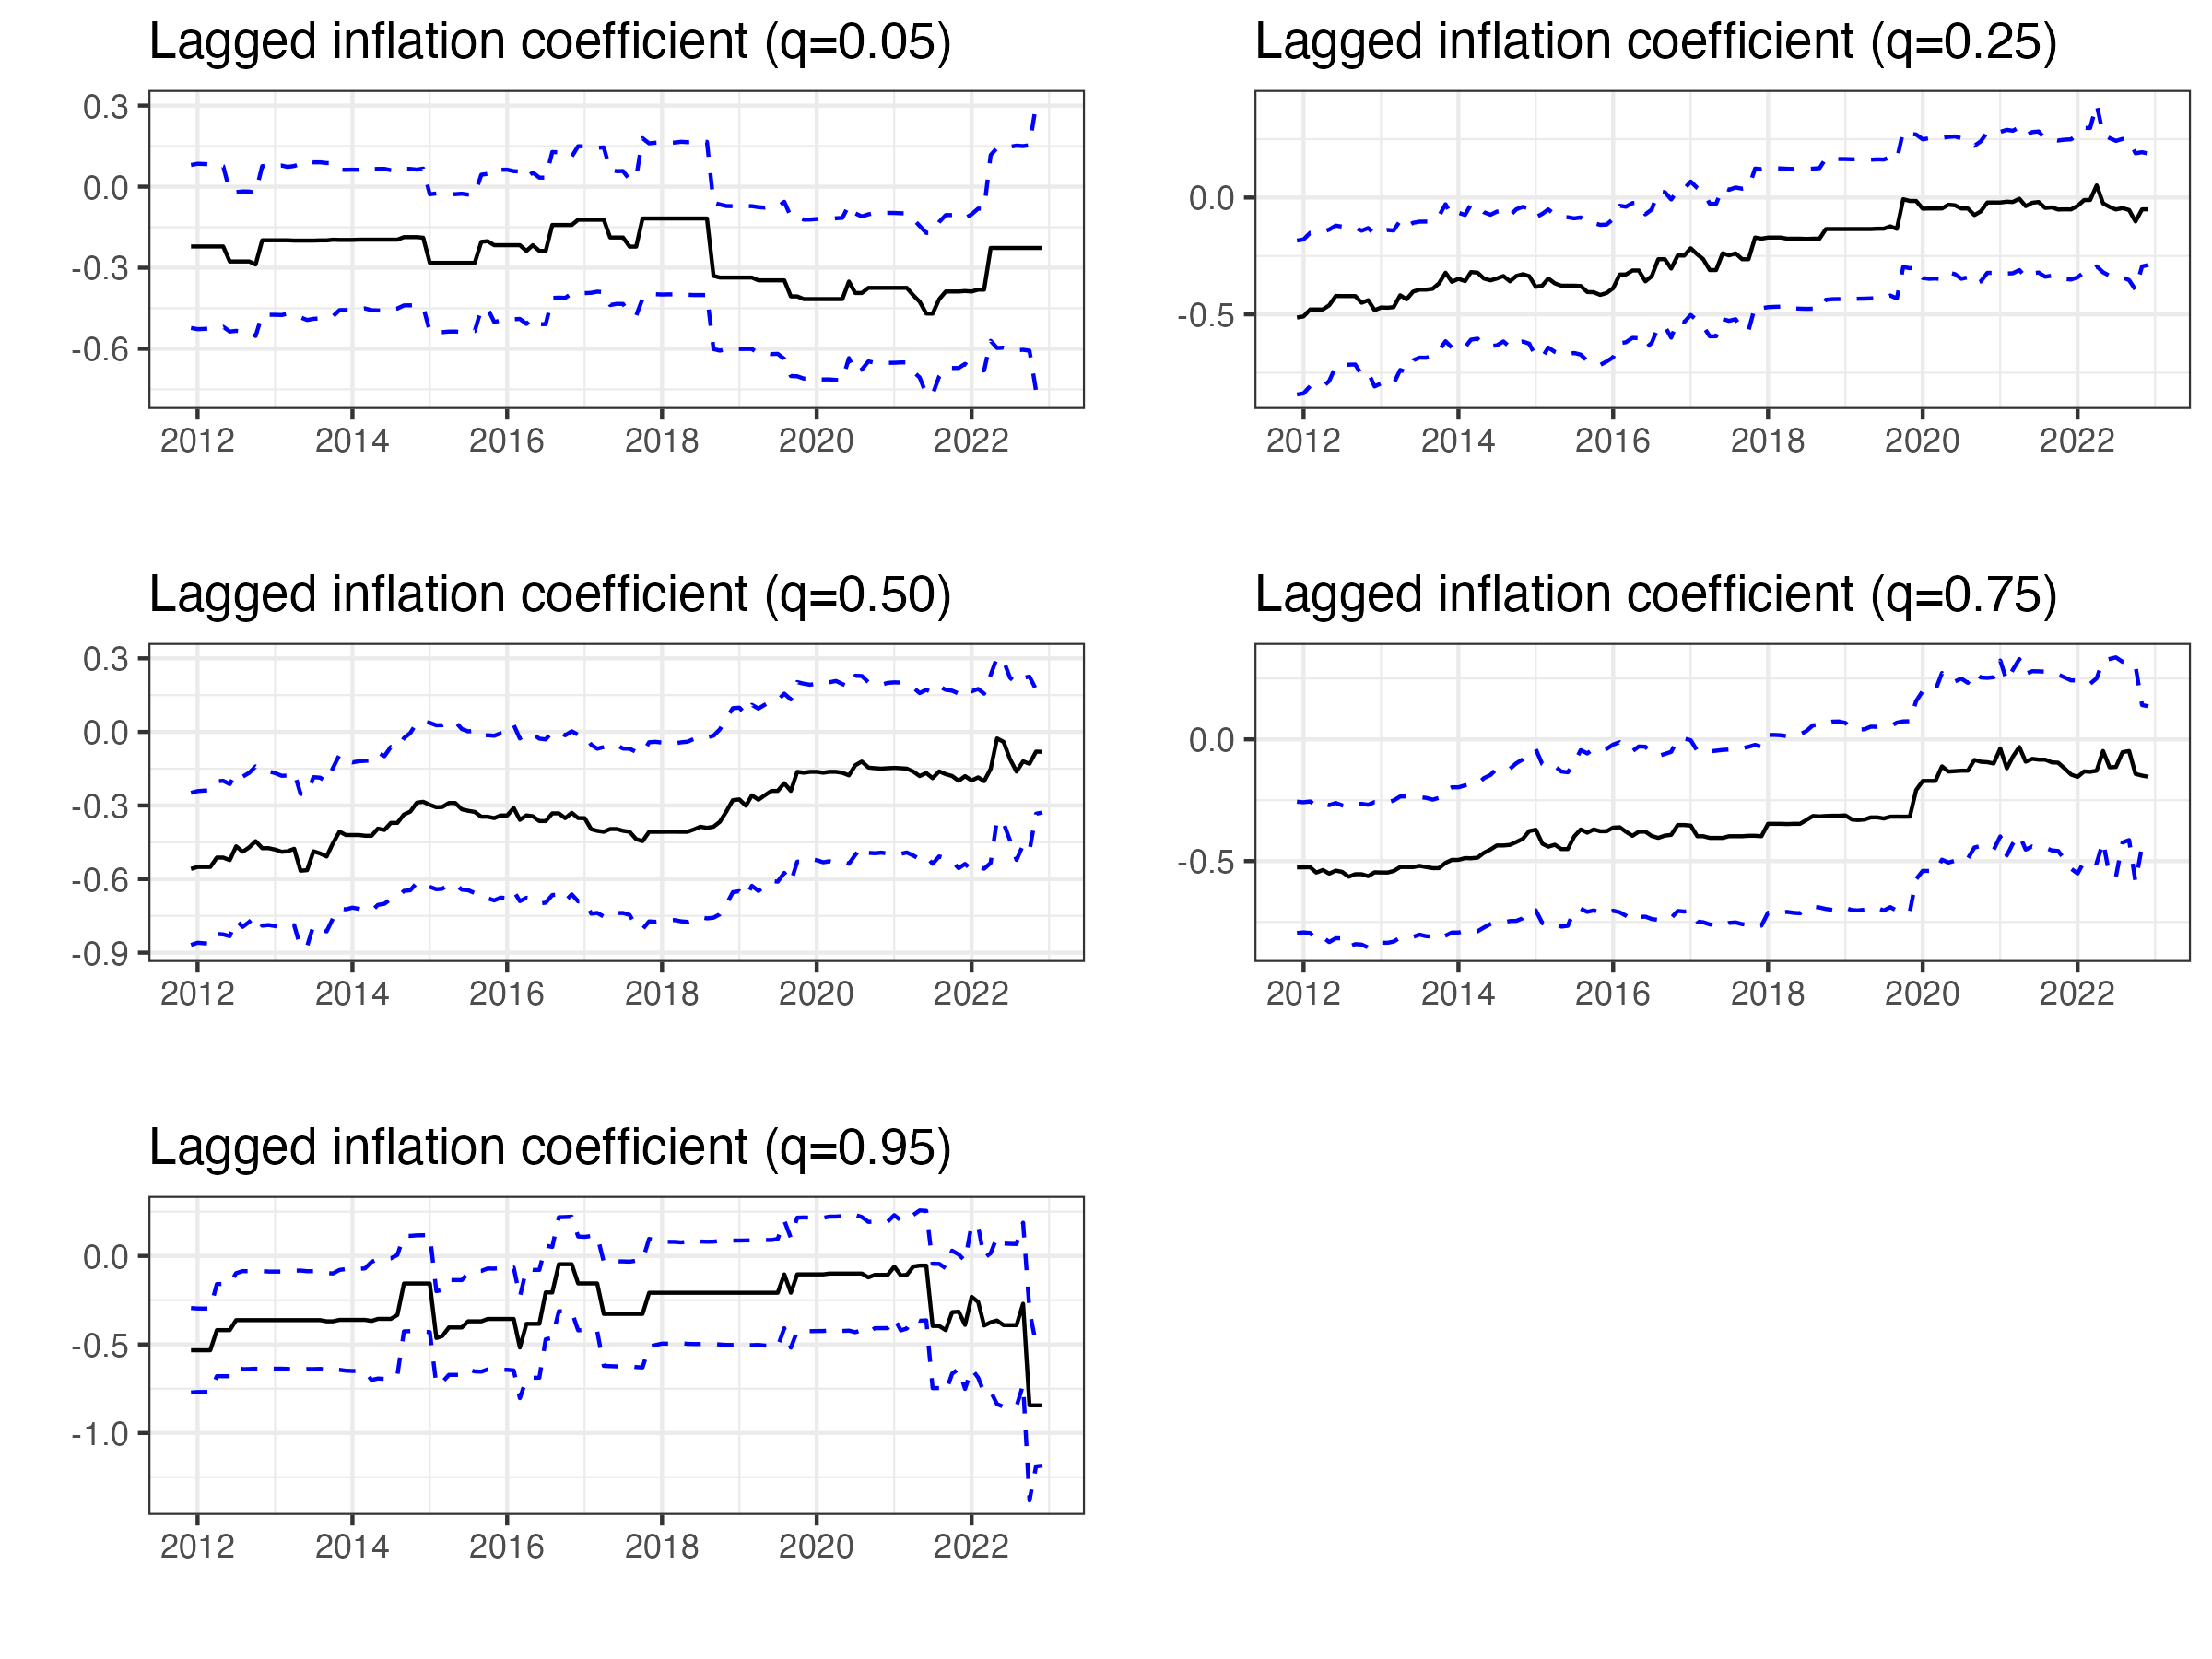}}
\subfigure[]{\includegraphics[width=0.30\textwidth]{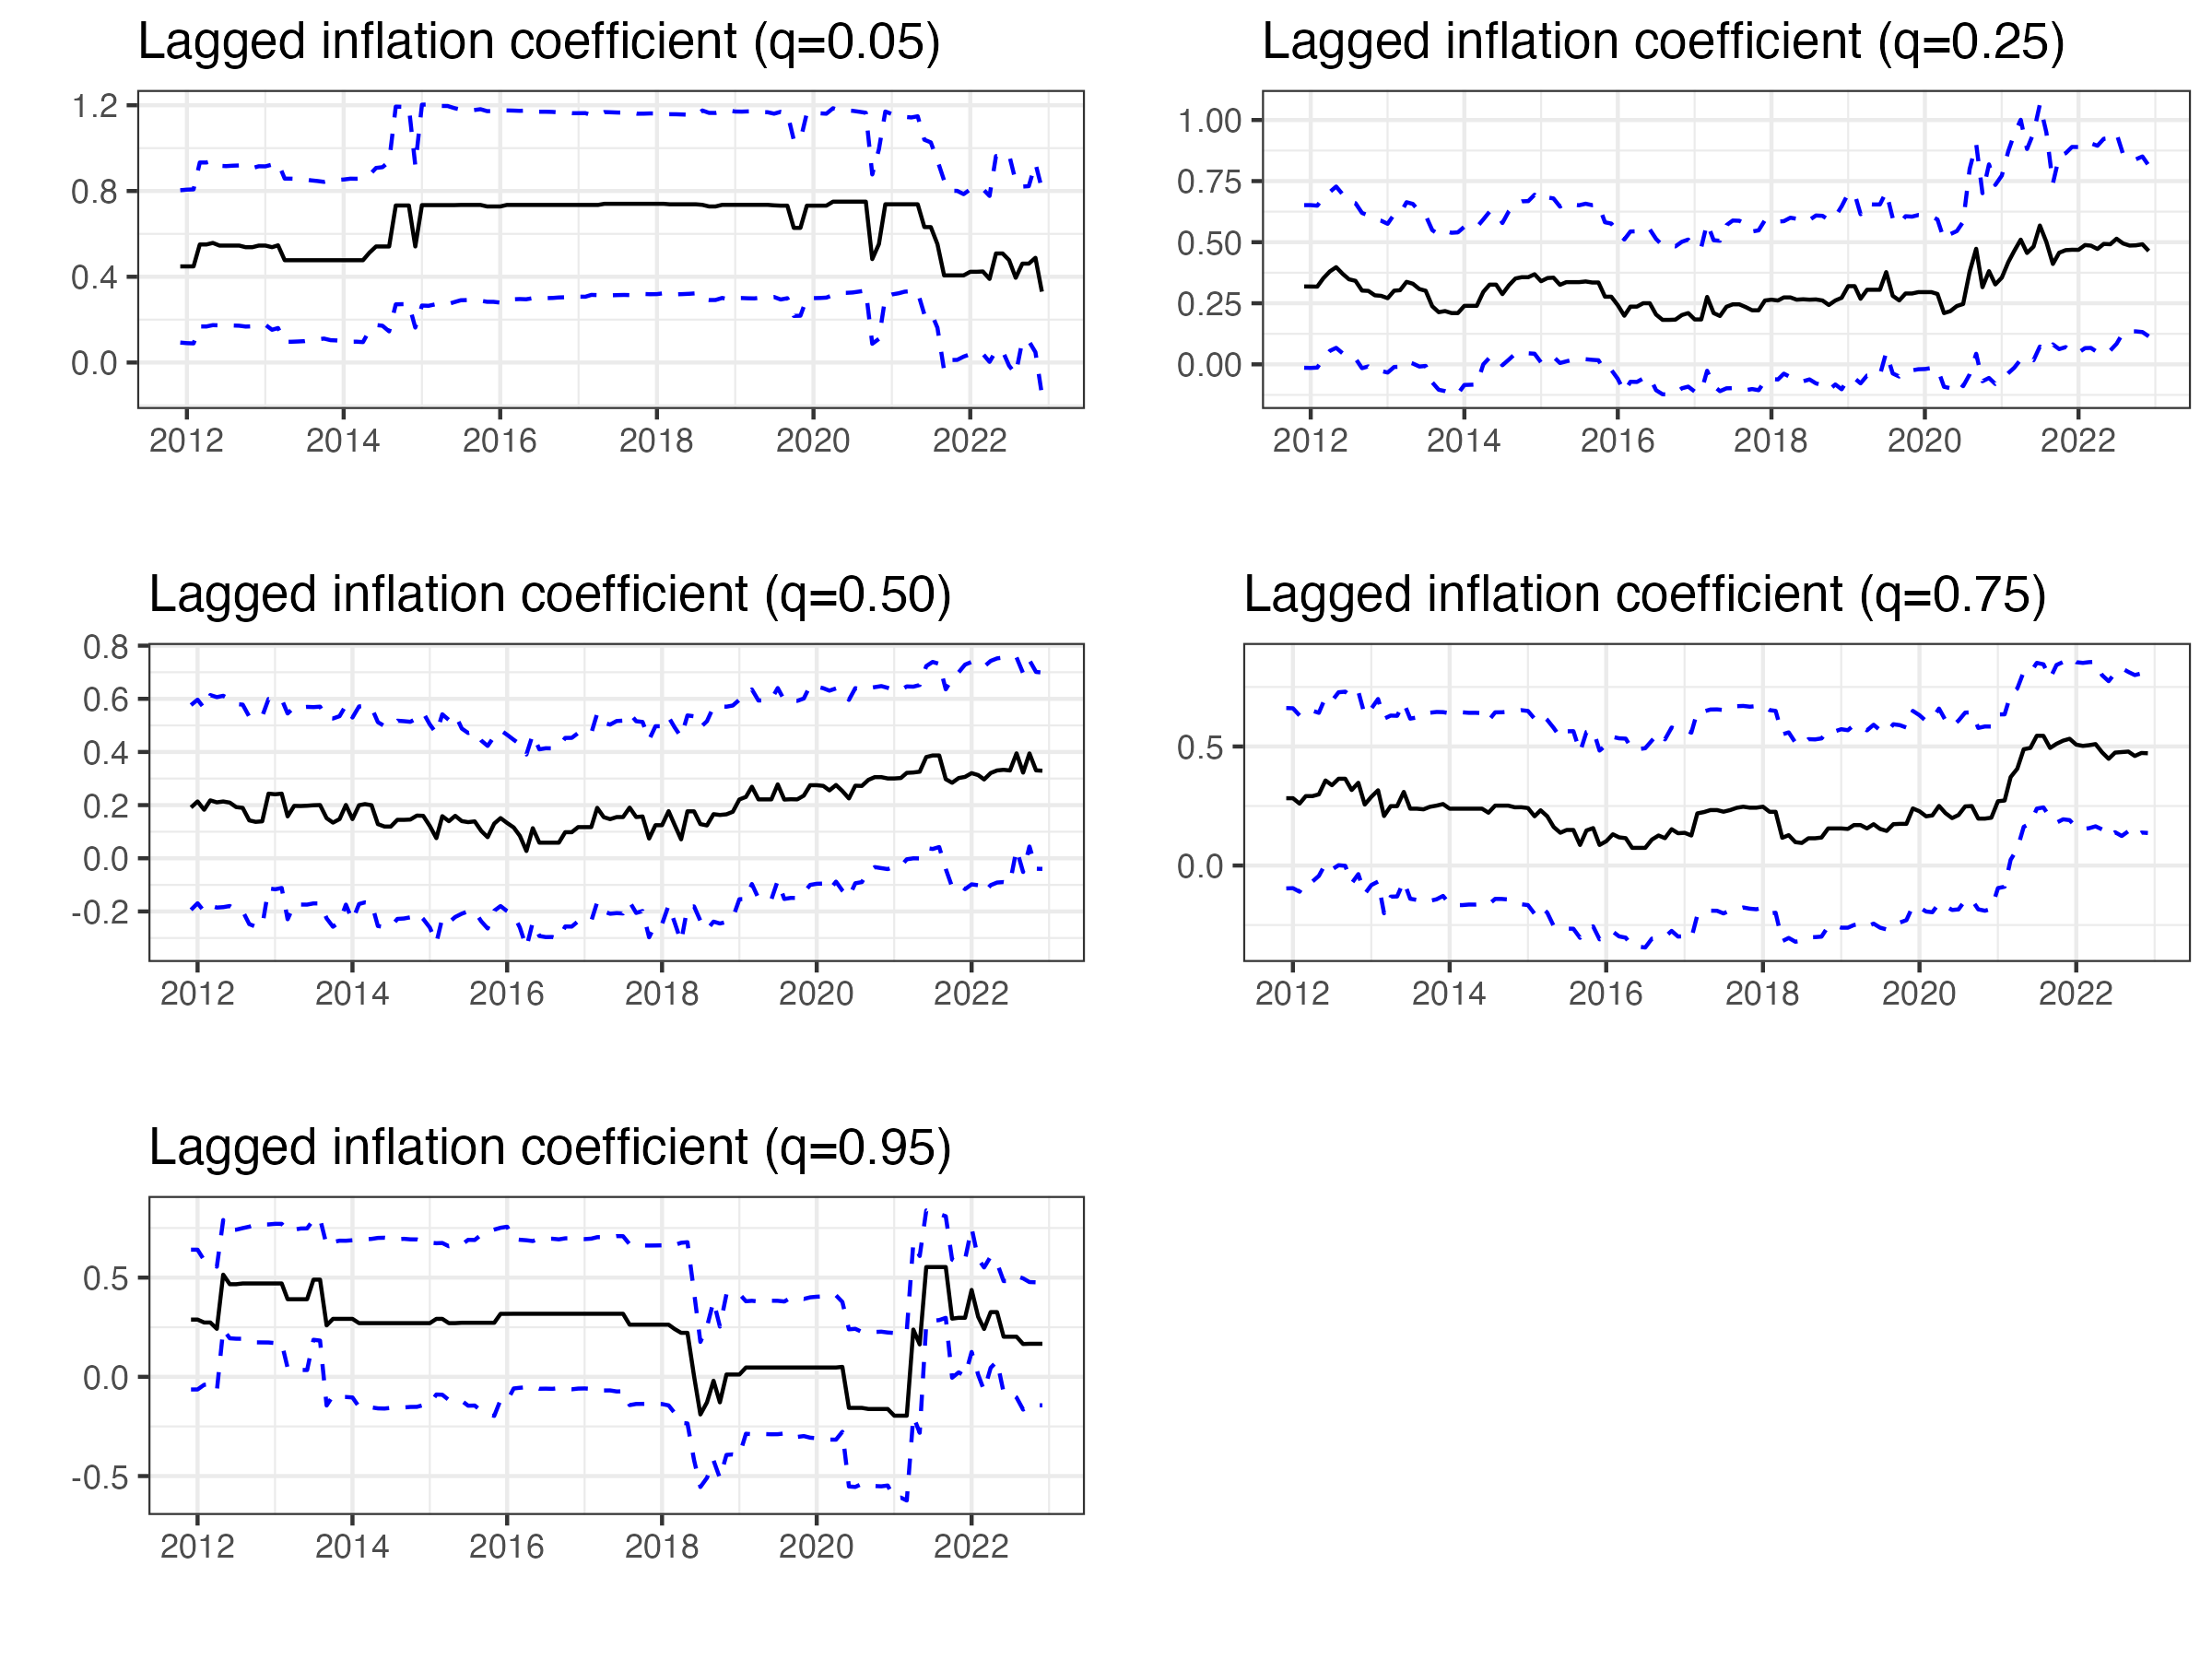}}
\subfigure[]{\includegraphics[width=0.30\textwidth]{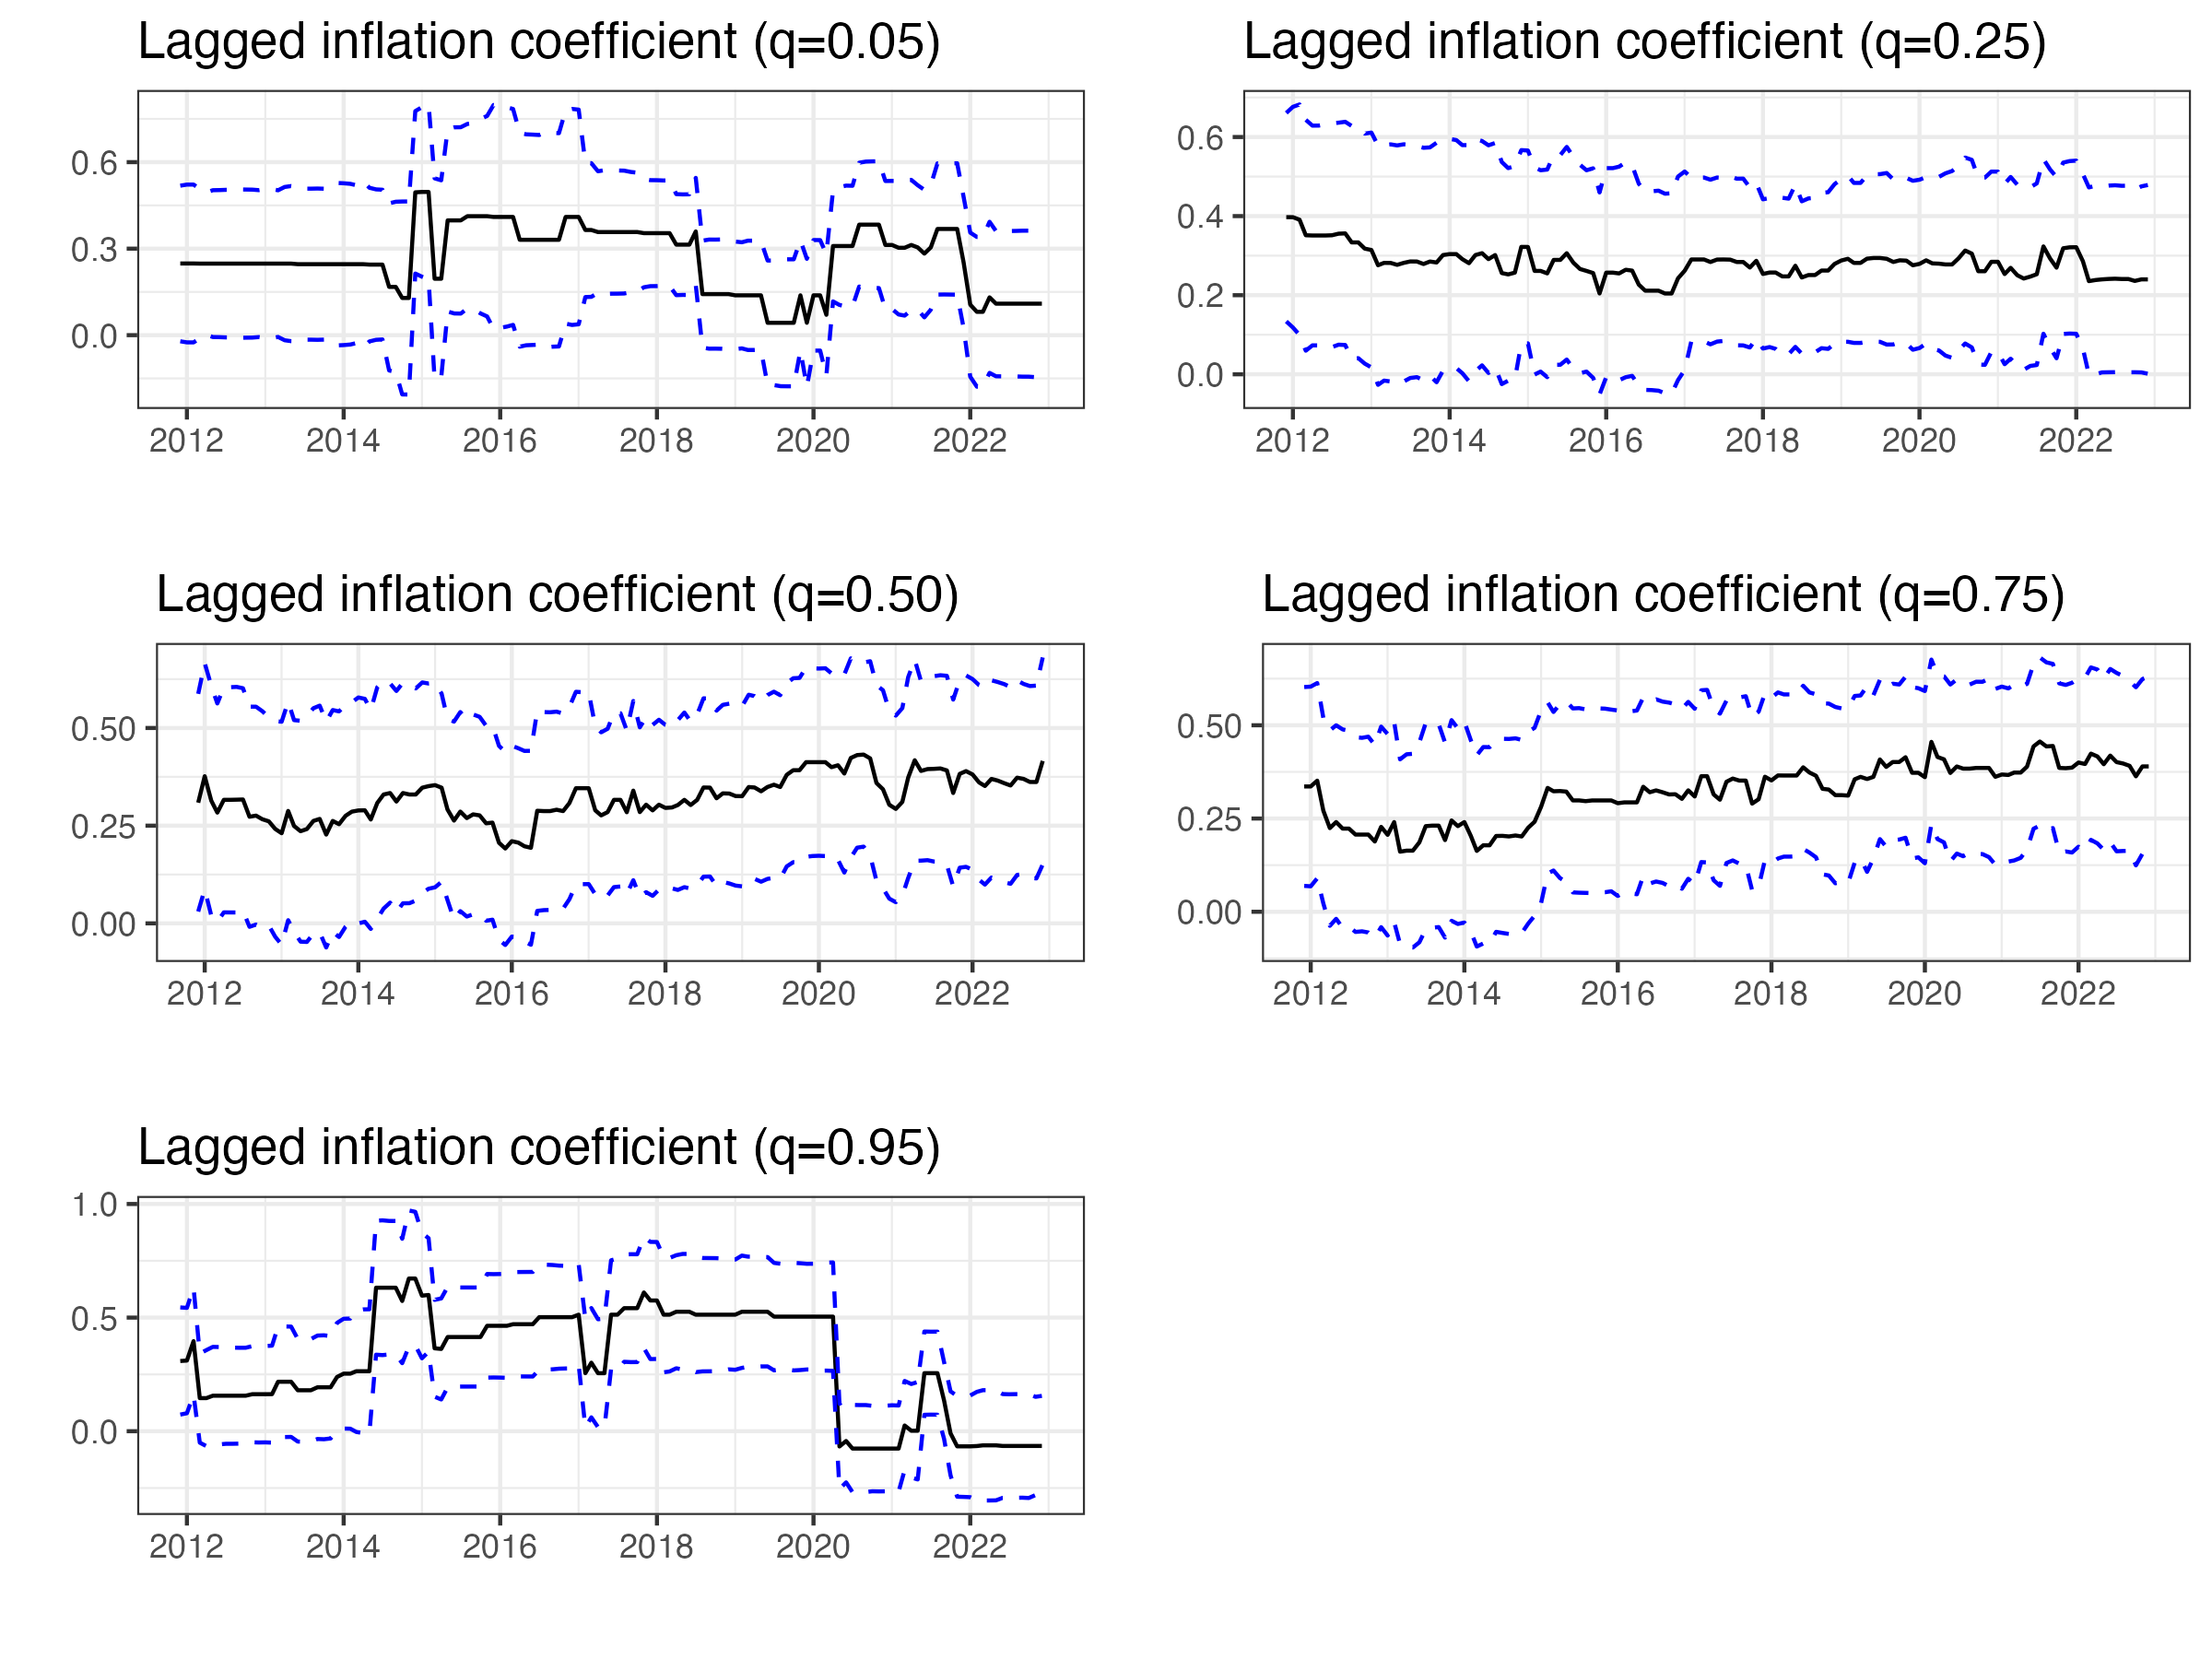}}\\
\subfigure[]{\includegraphics[width=0.30\textwidth]{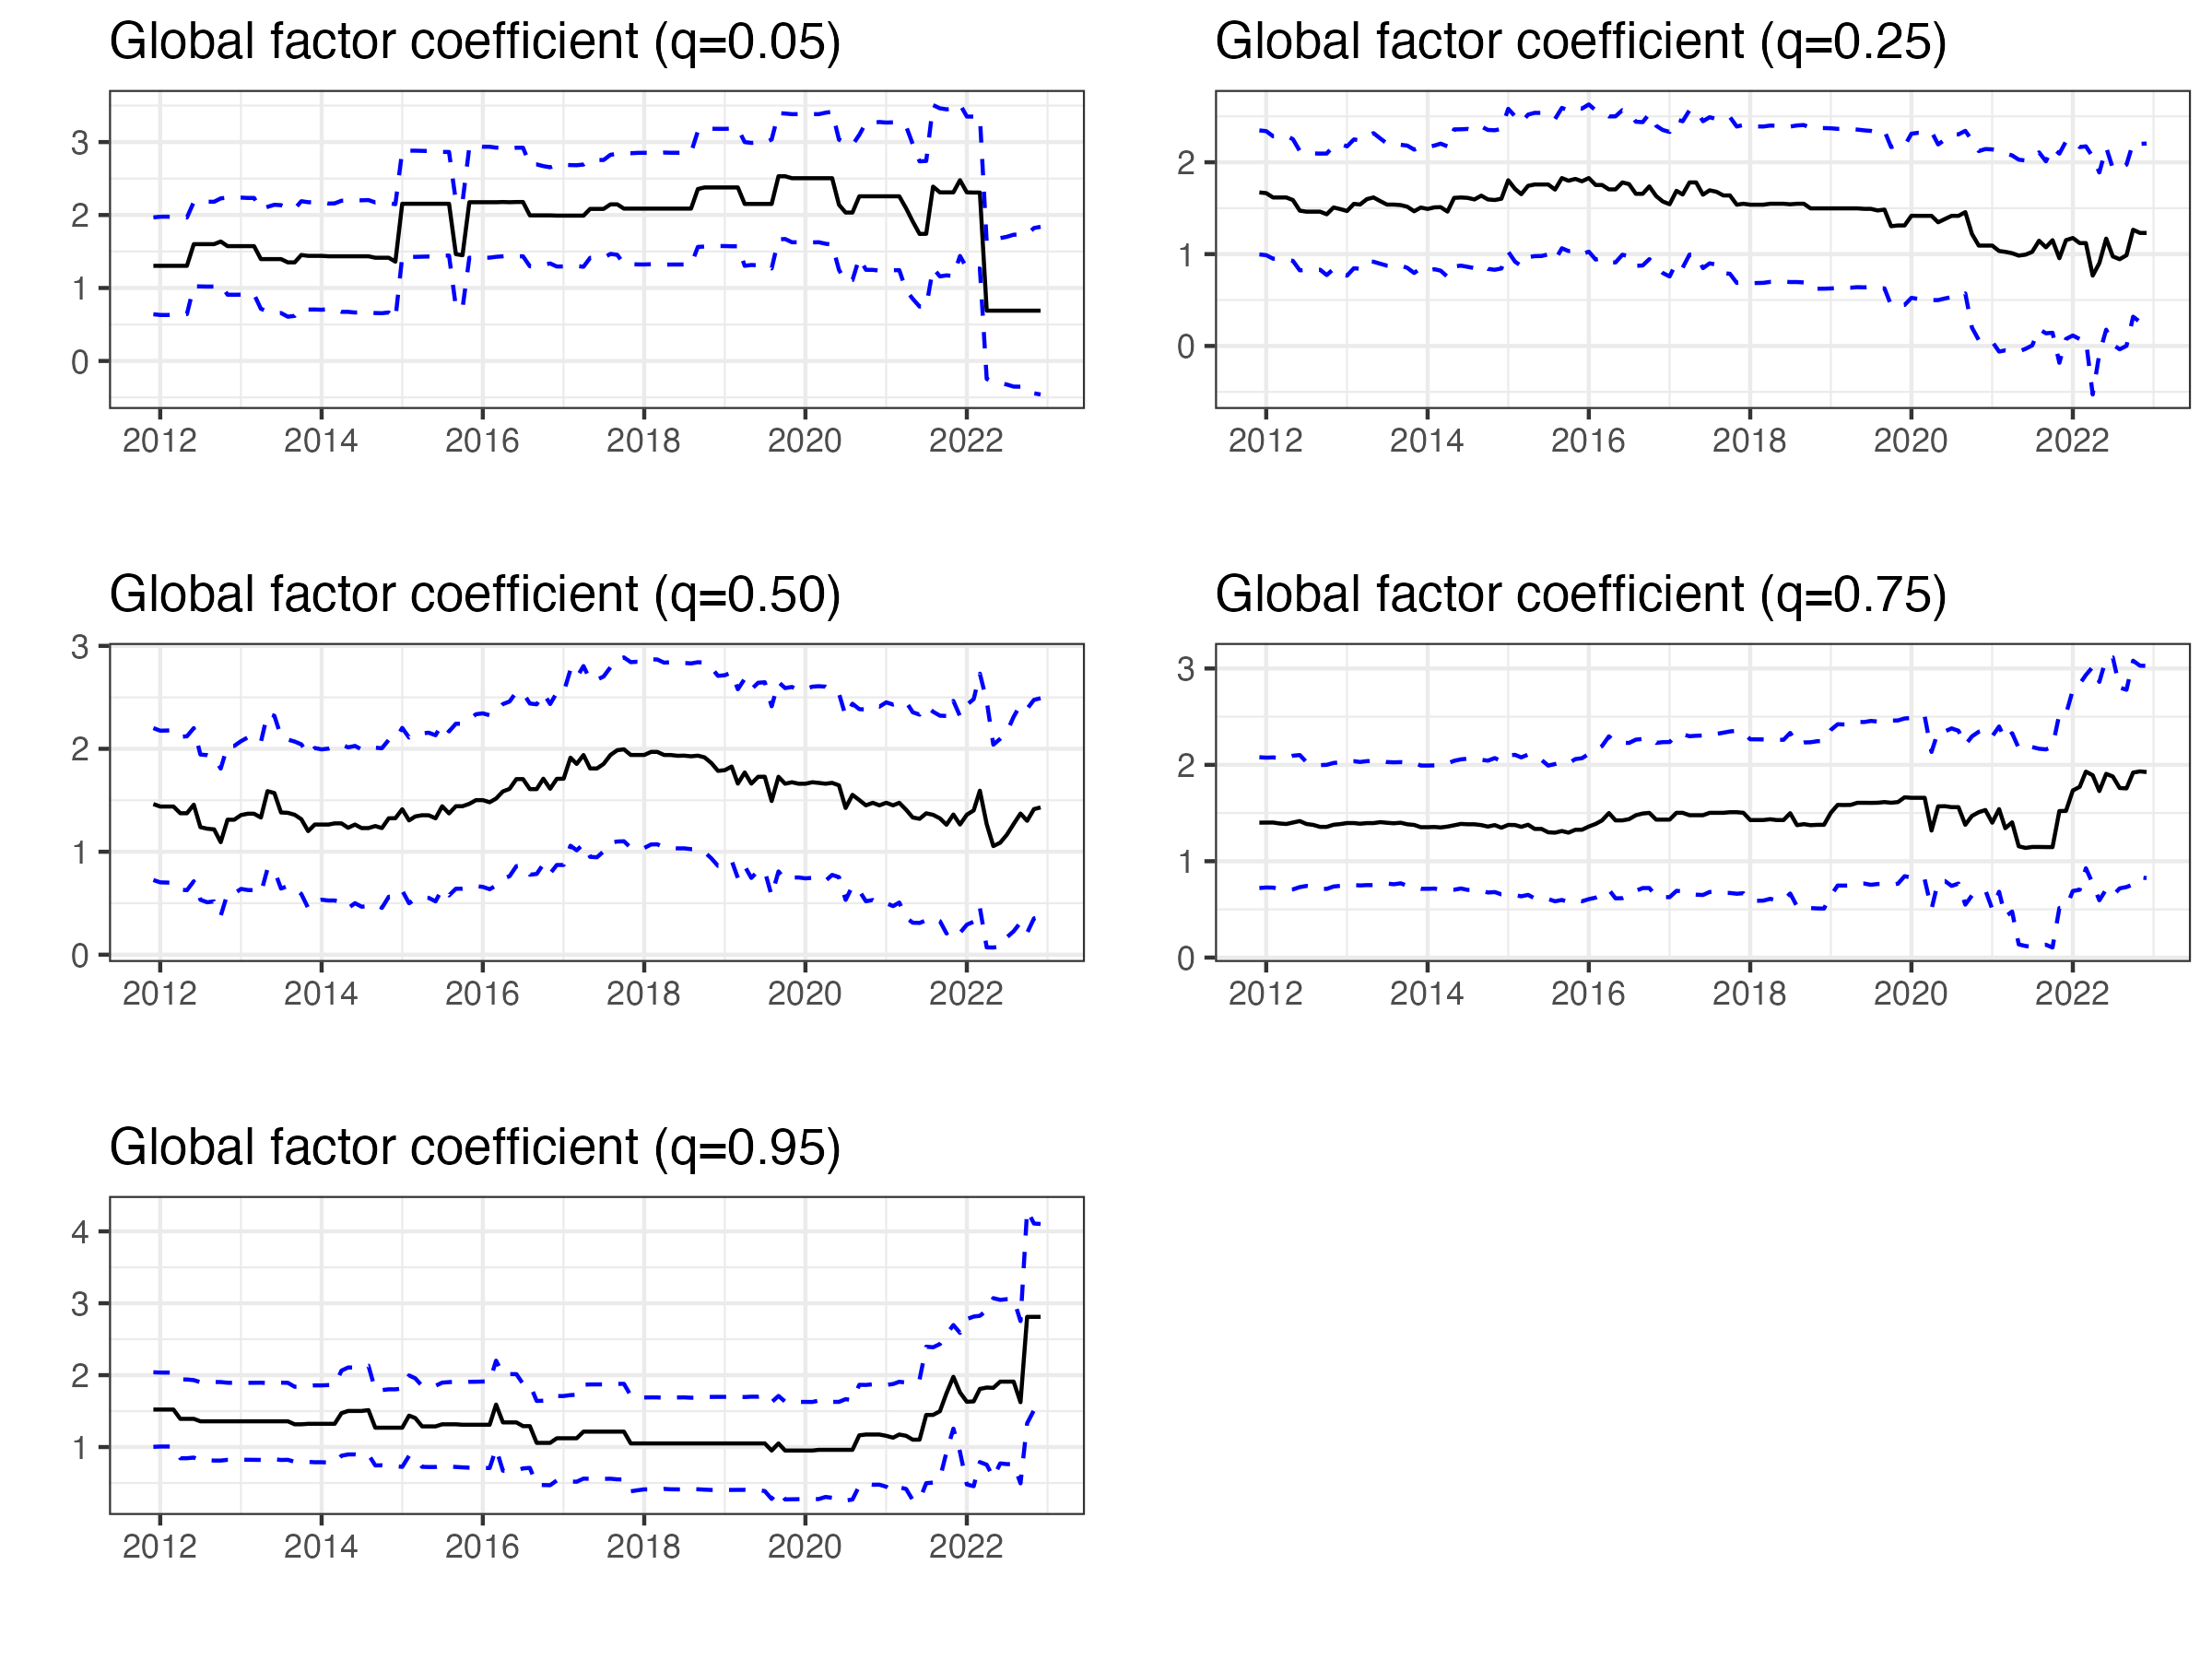}}
\subfigure[]{\includegraphics[width=0.30\textwidth]{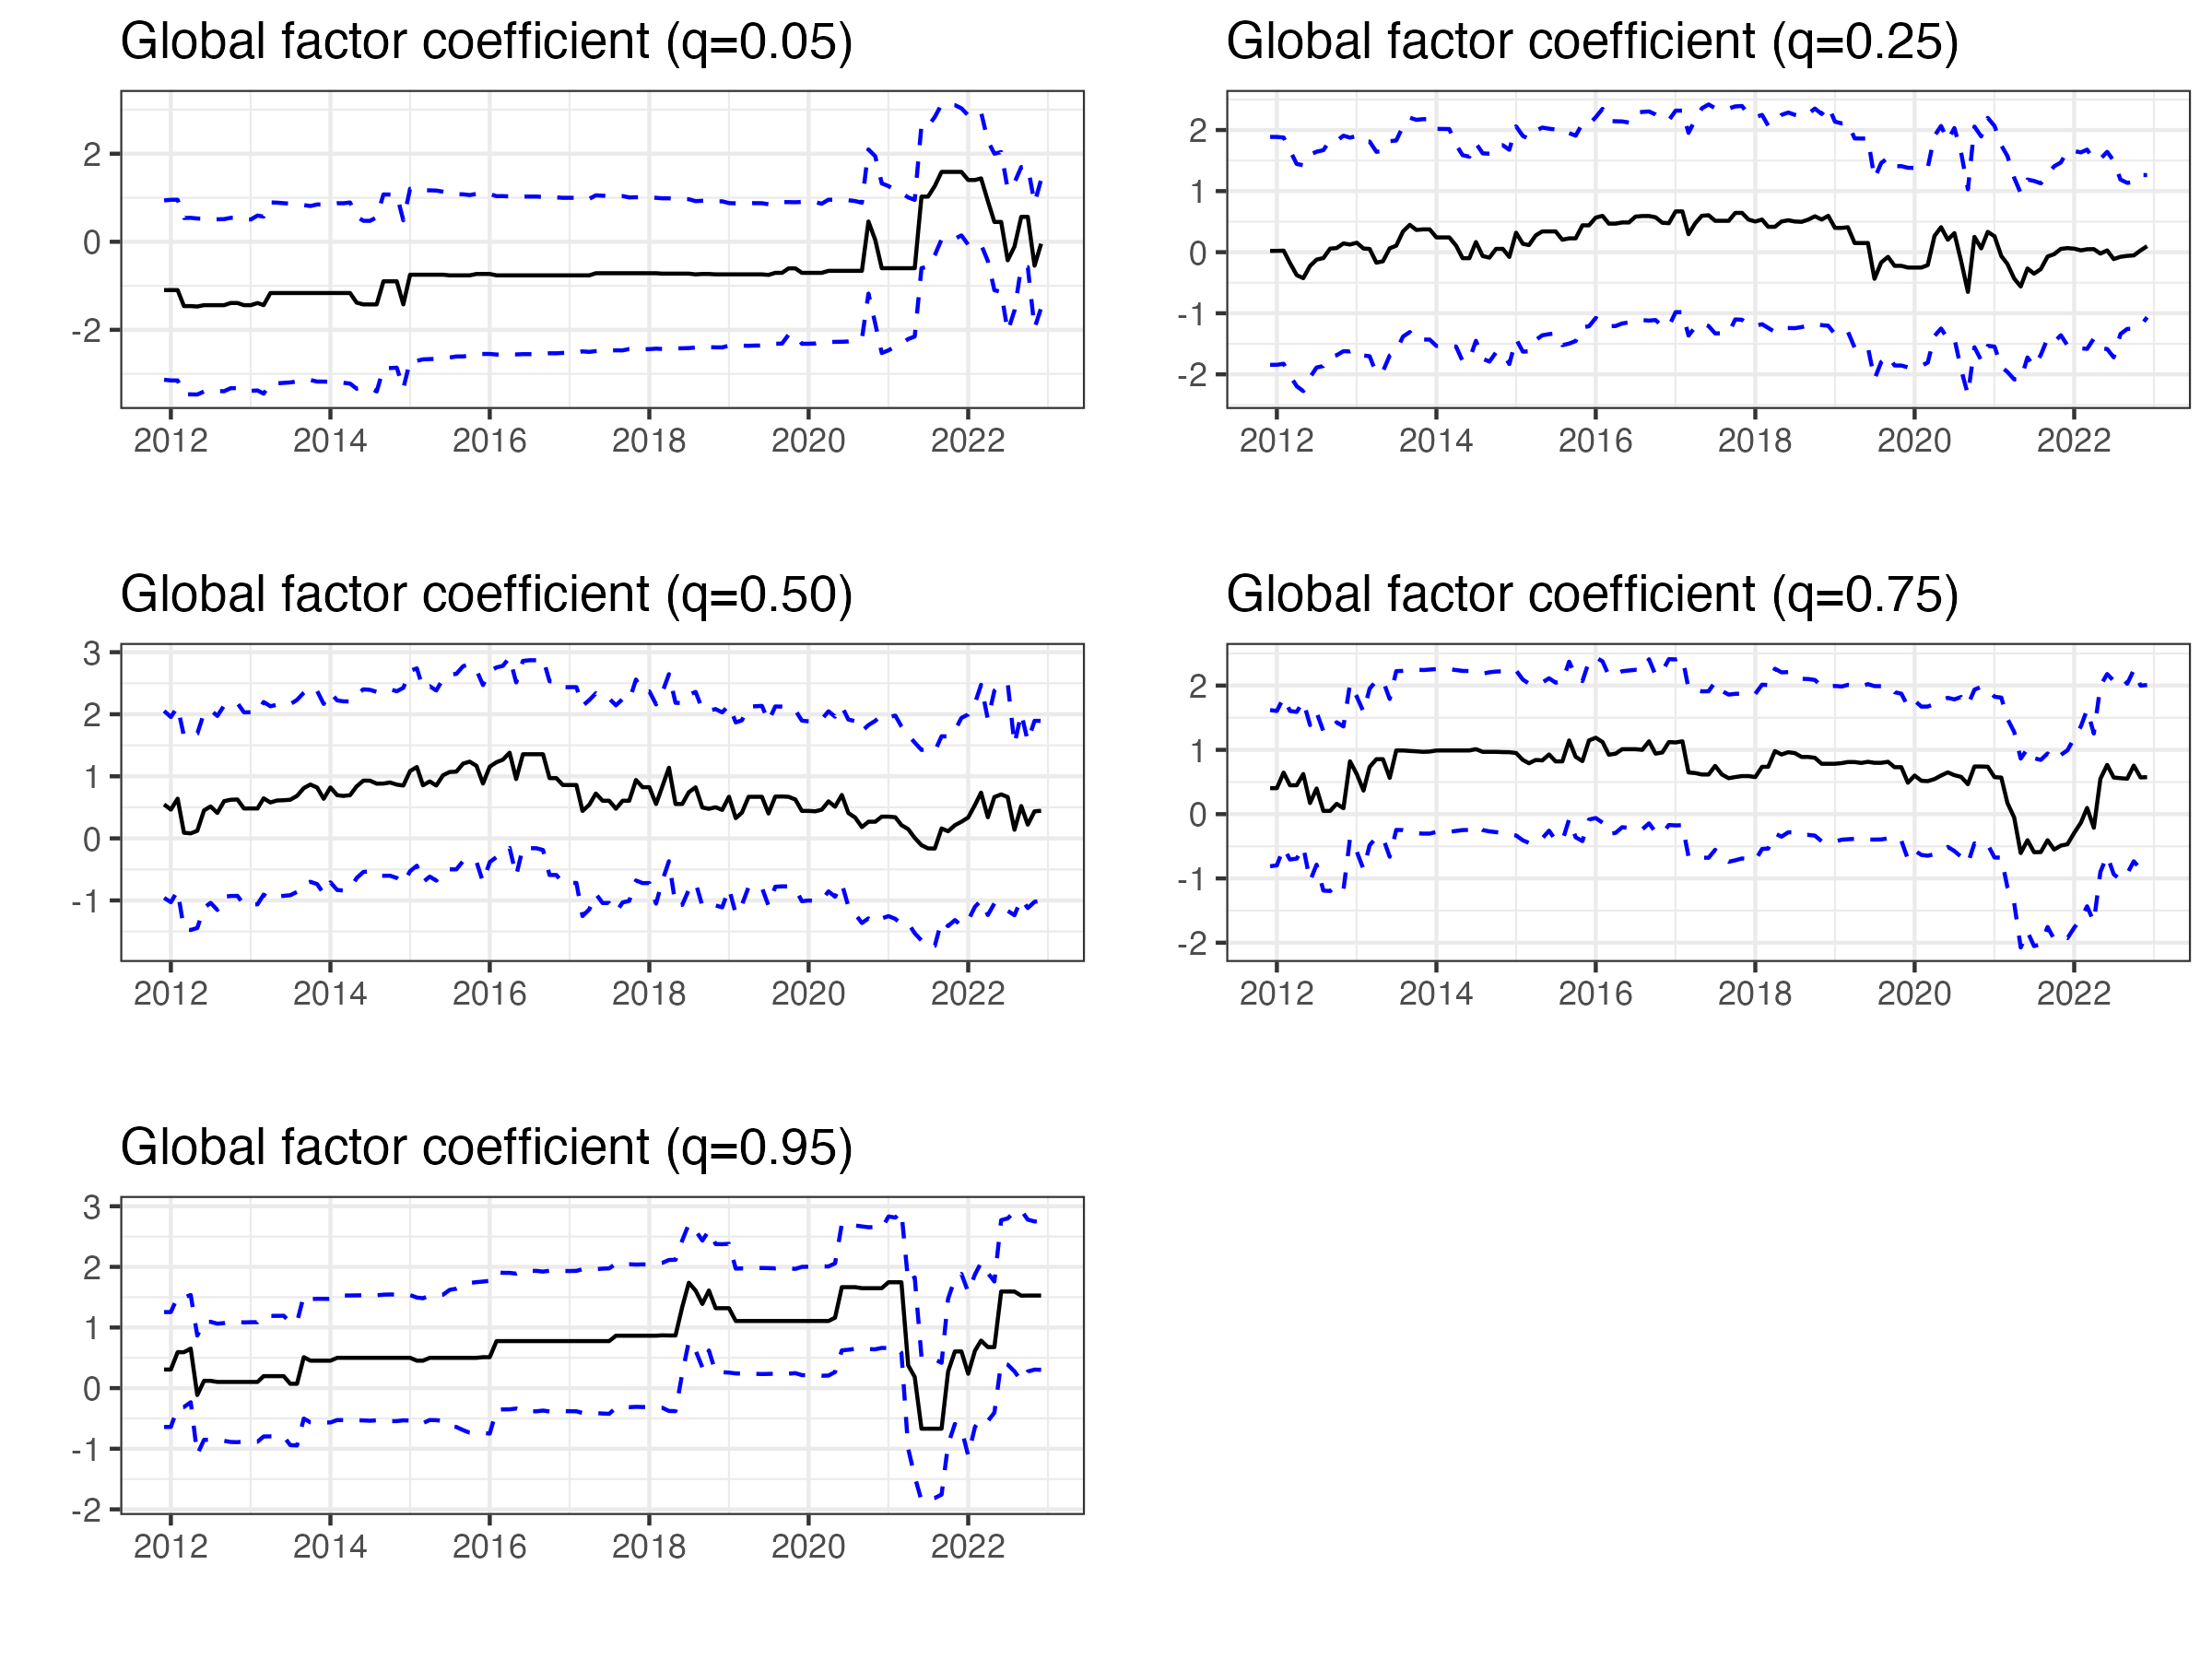}}
\subfigure[]{\includegraphics[width=0.30\textwidth]{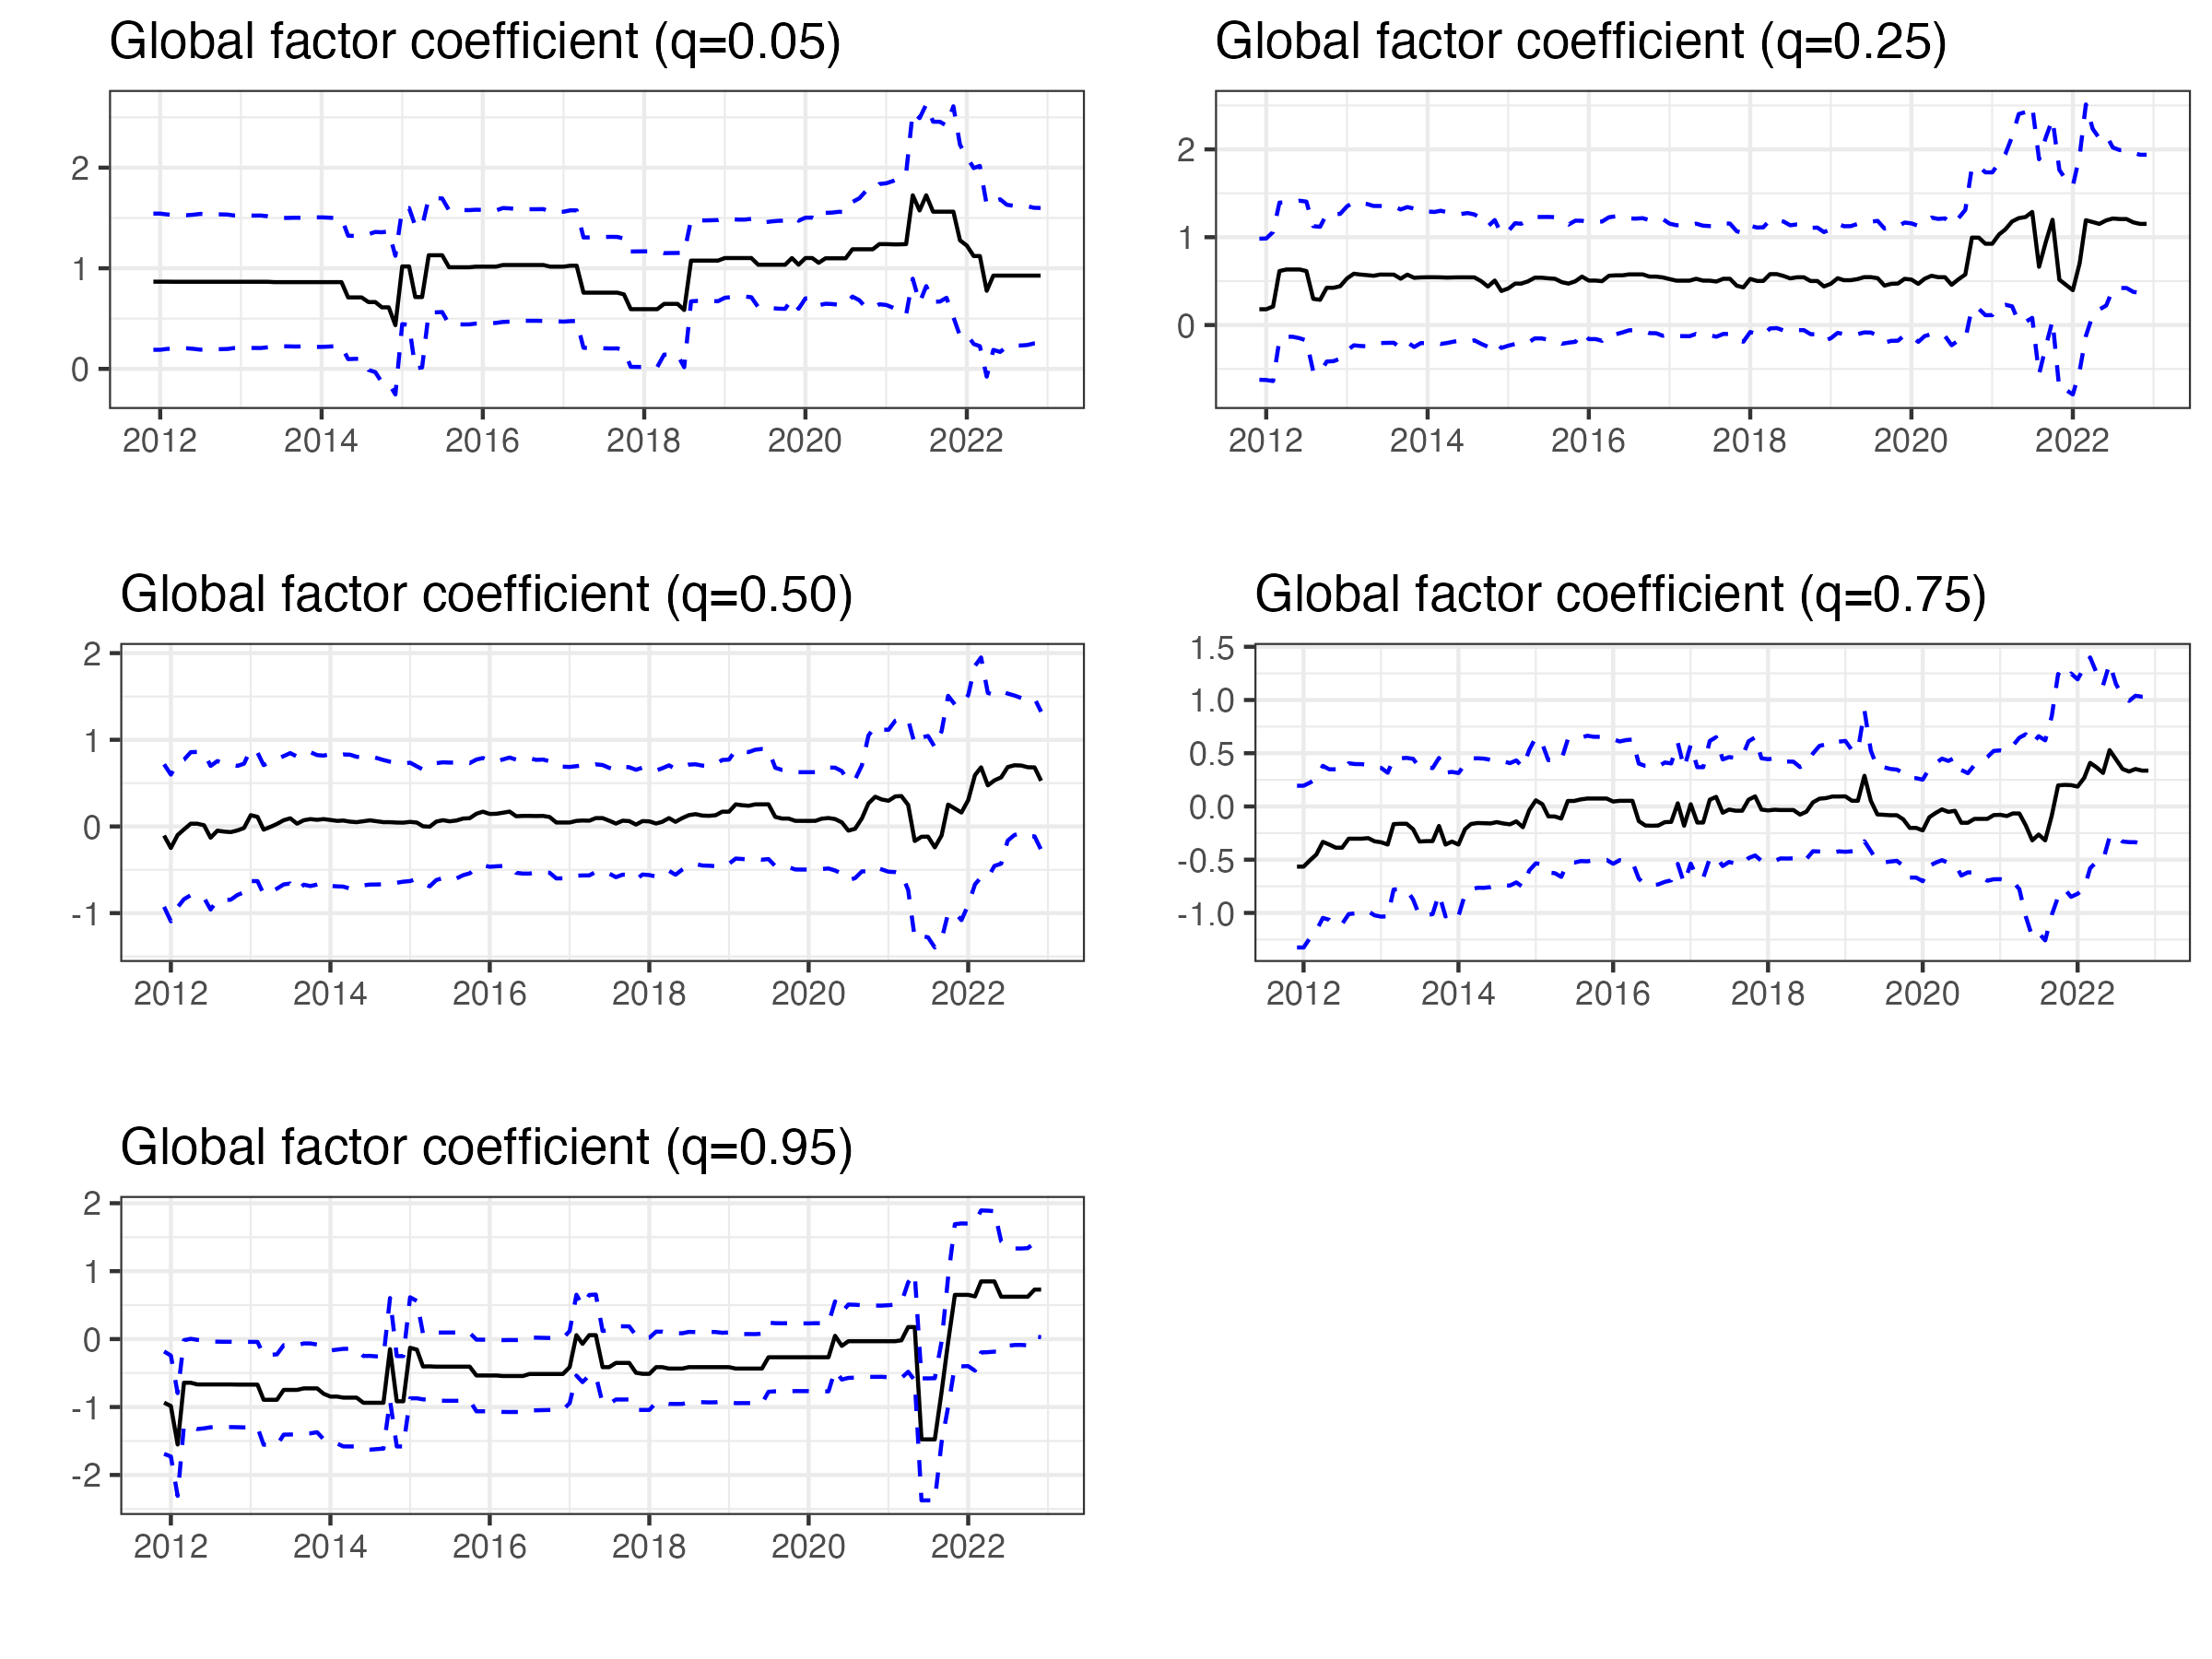}}\\
\subfigure[]{\includegraphics[width=0.3\textwidth]{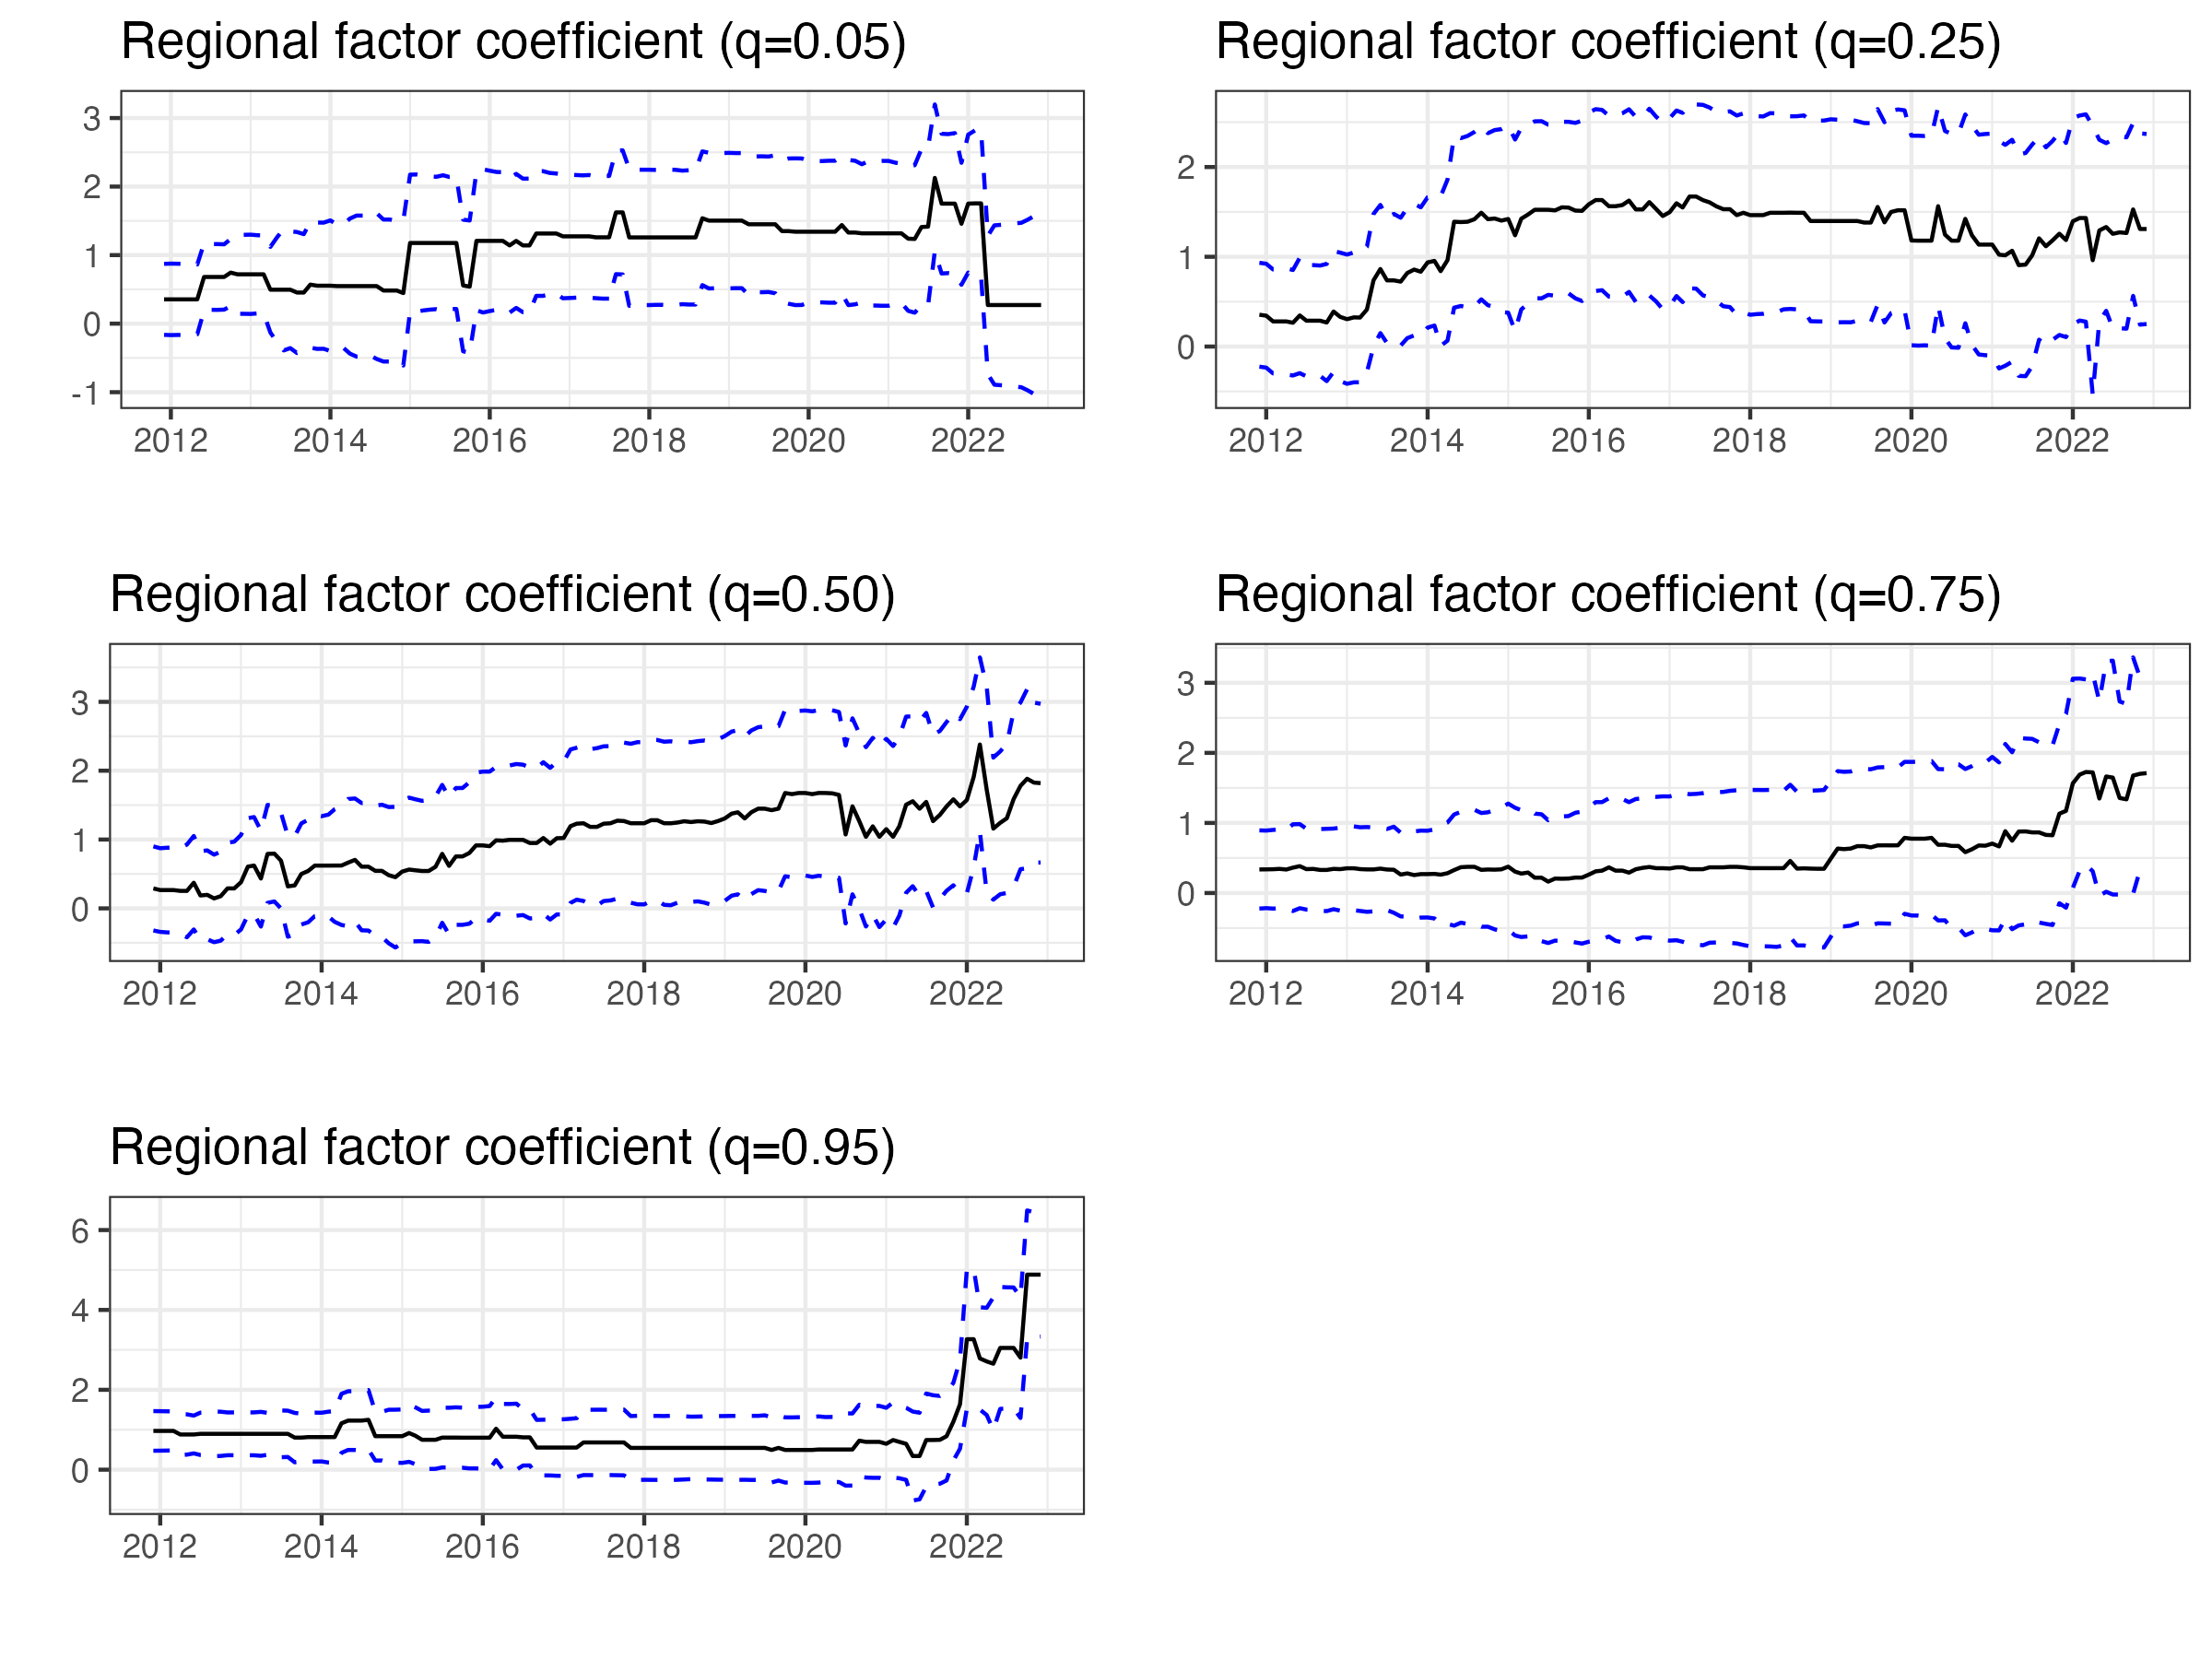}}
\subfigure[]{\includegraphics[width=0.3\textwidth]{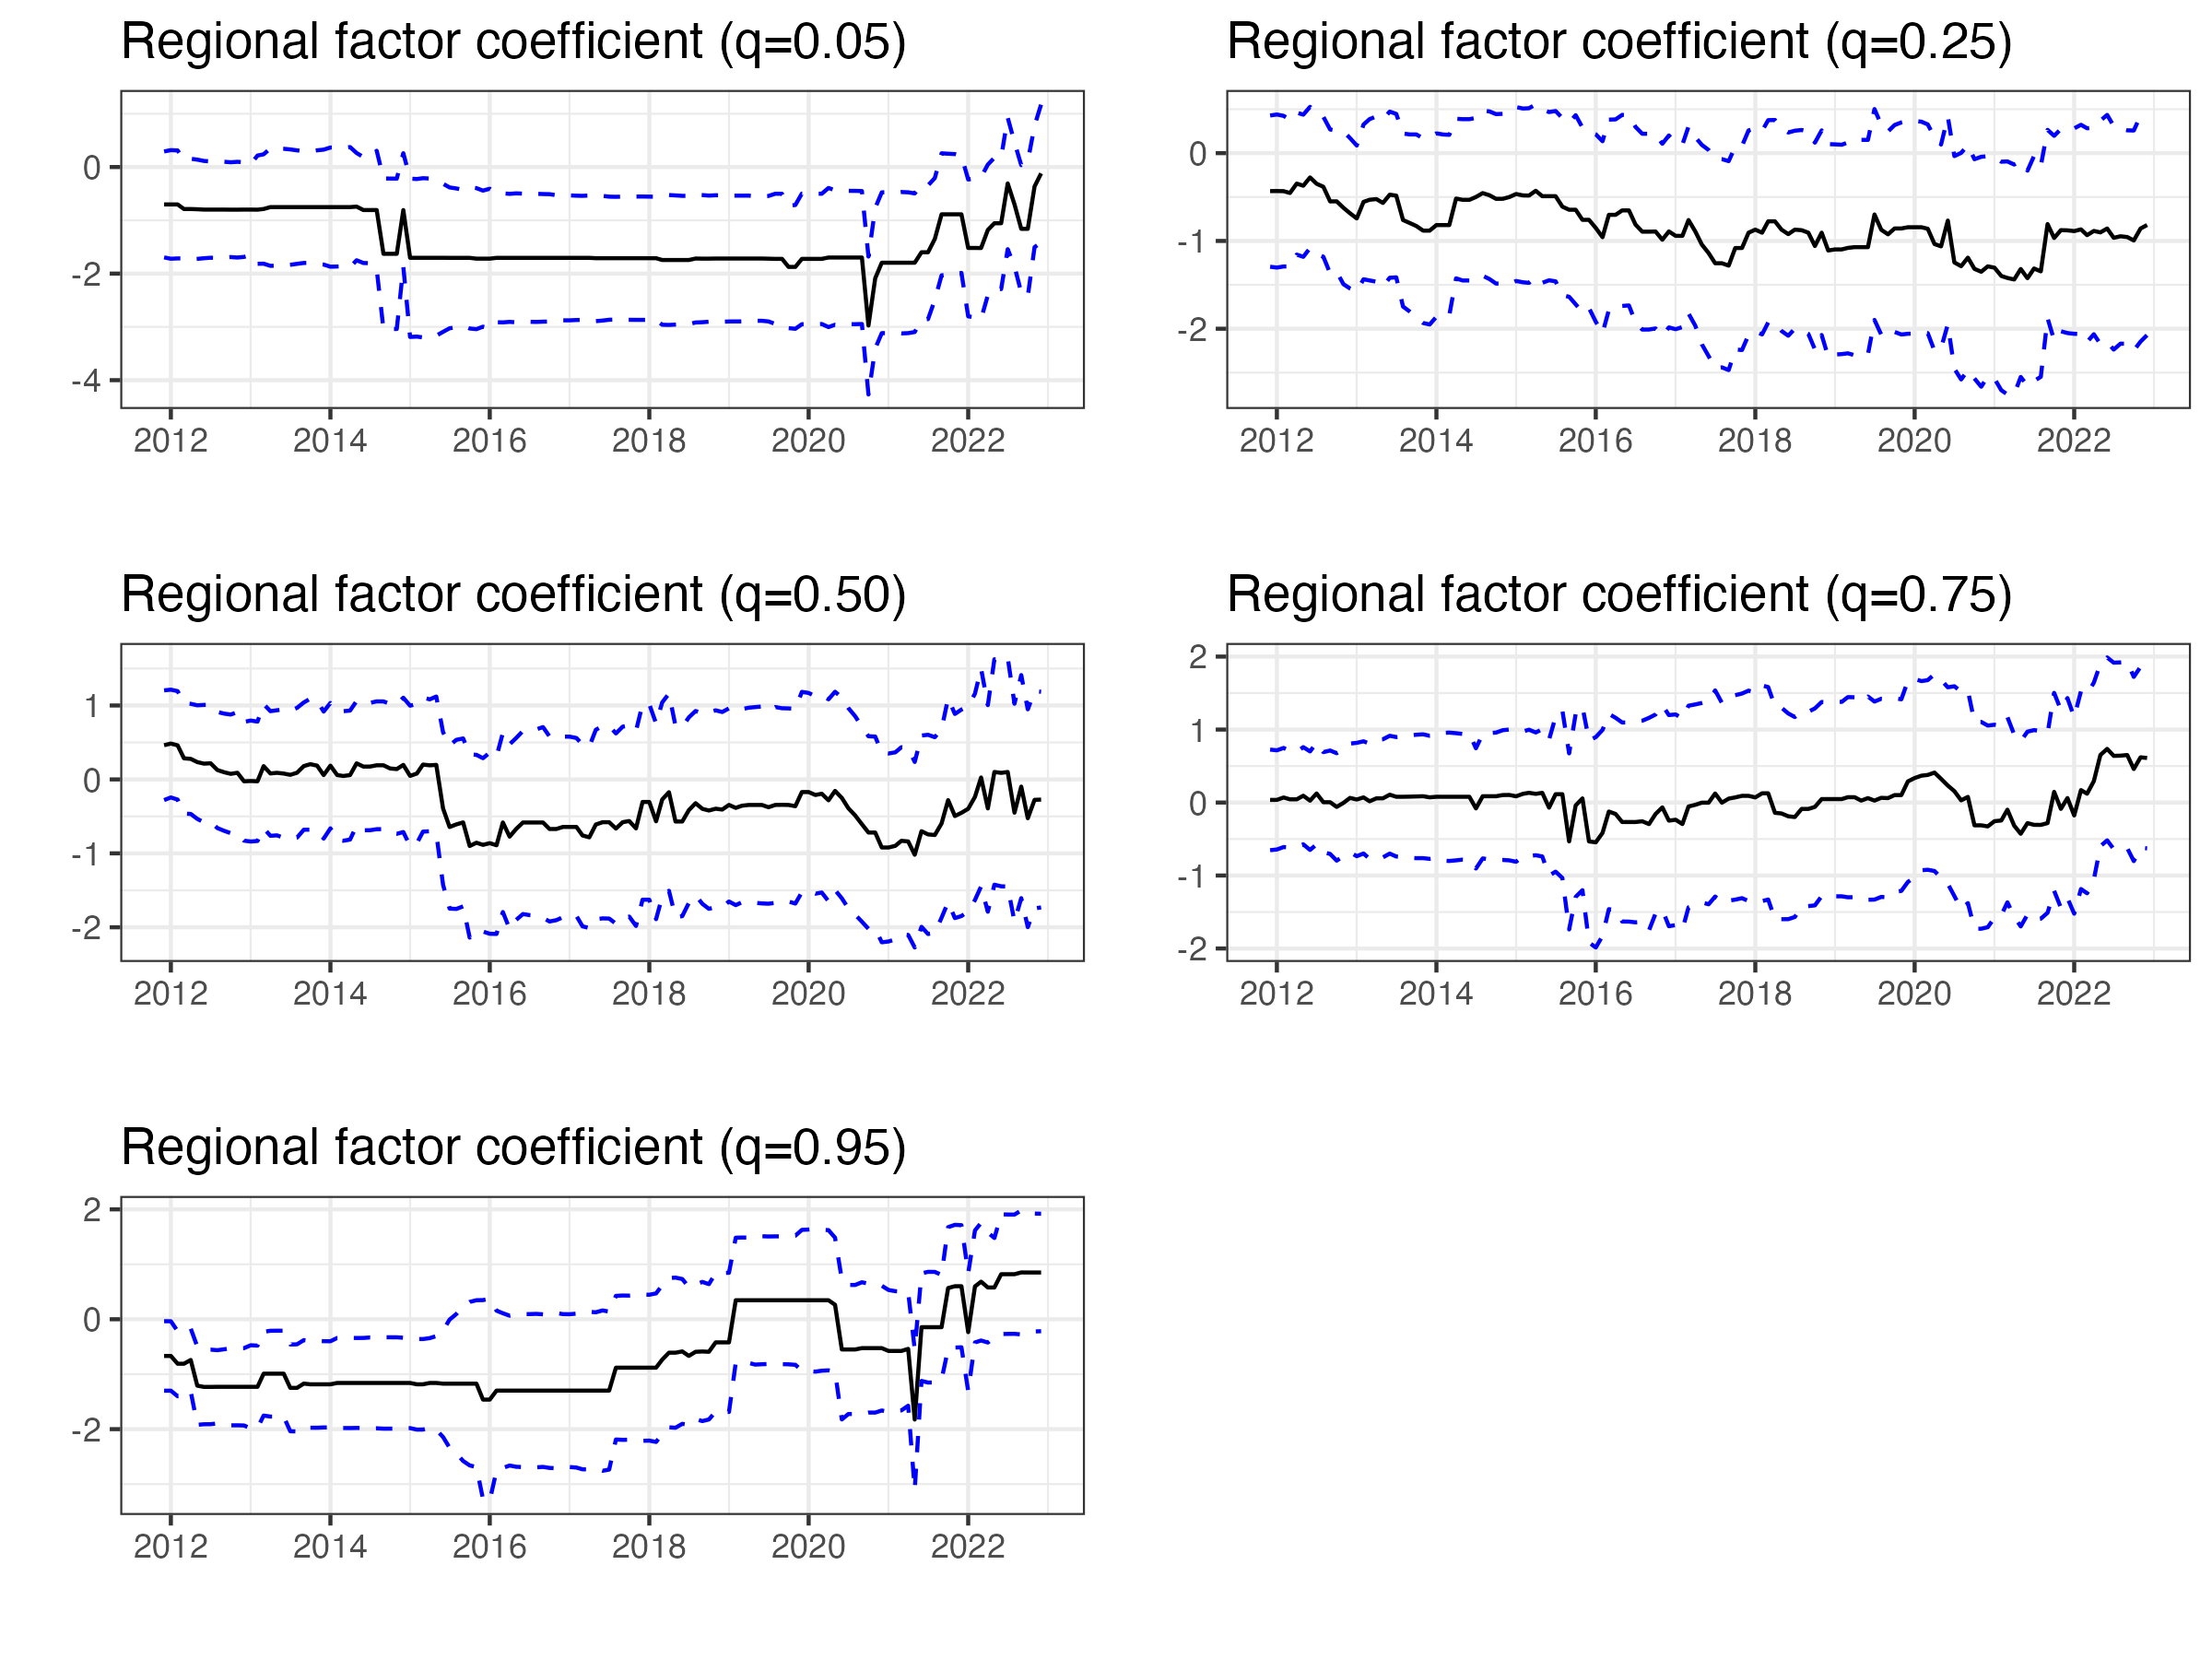}}
\subfigure[]{\includegraphics[width=0.3\textwidth]{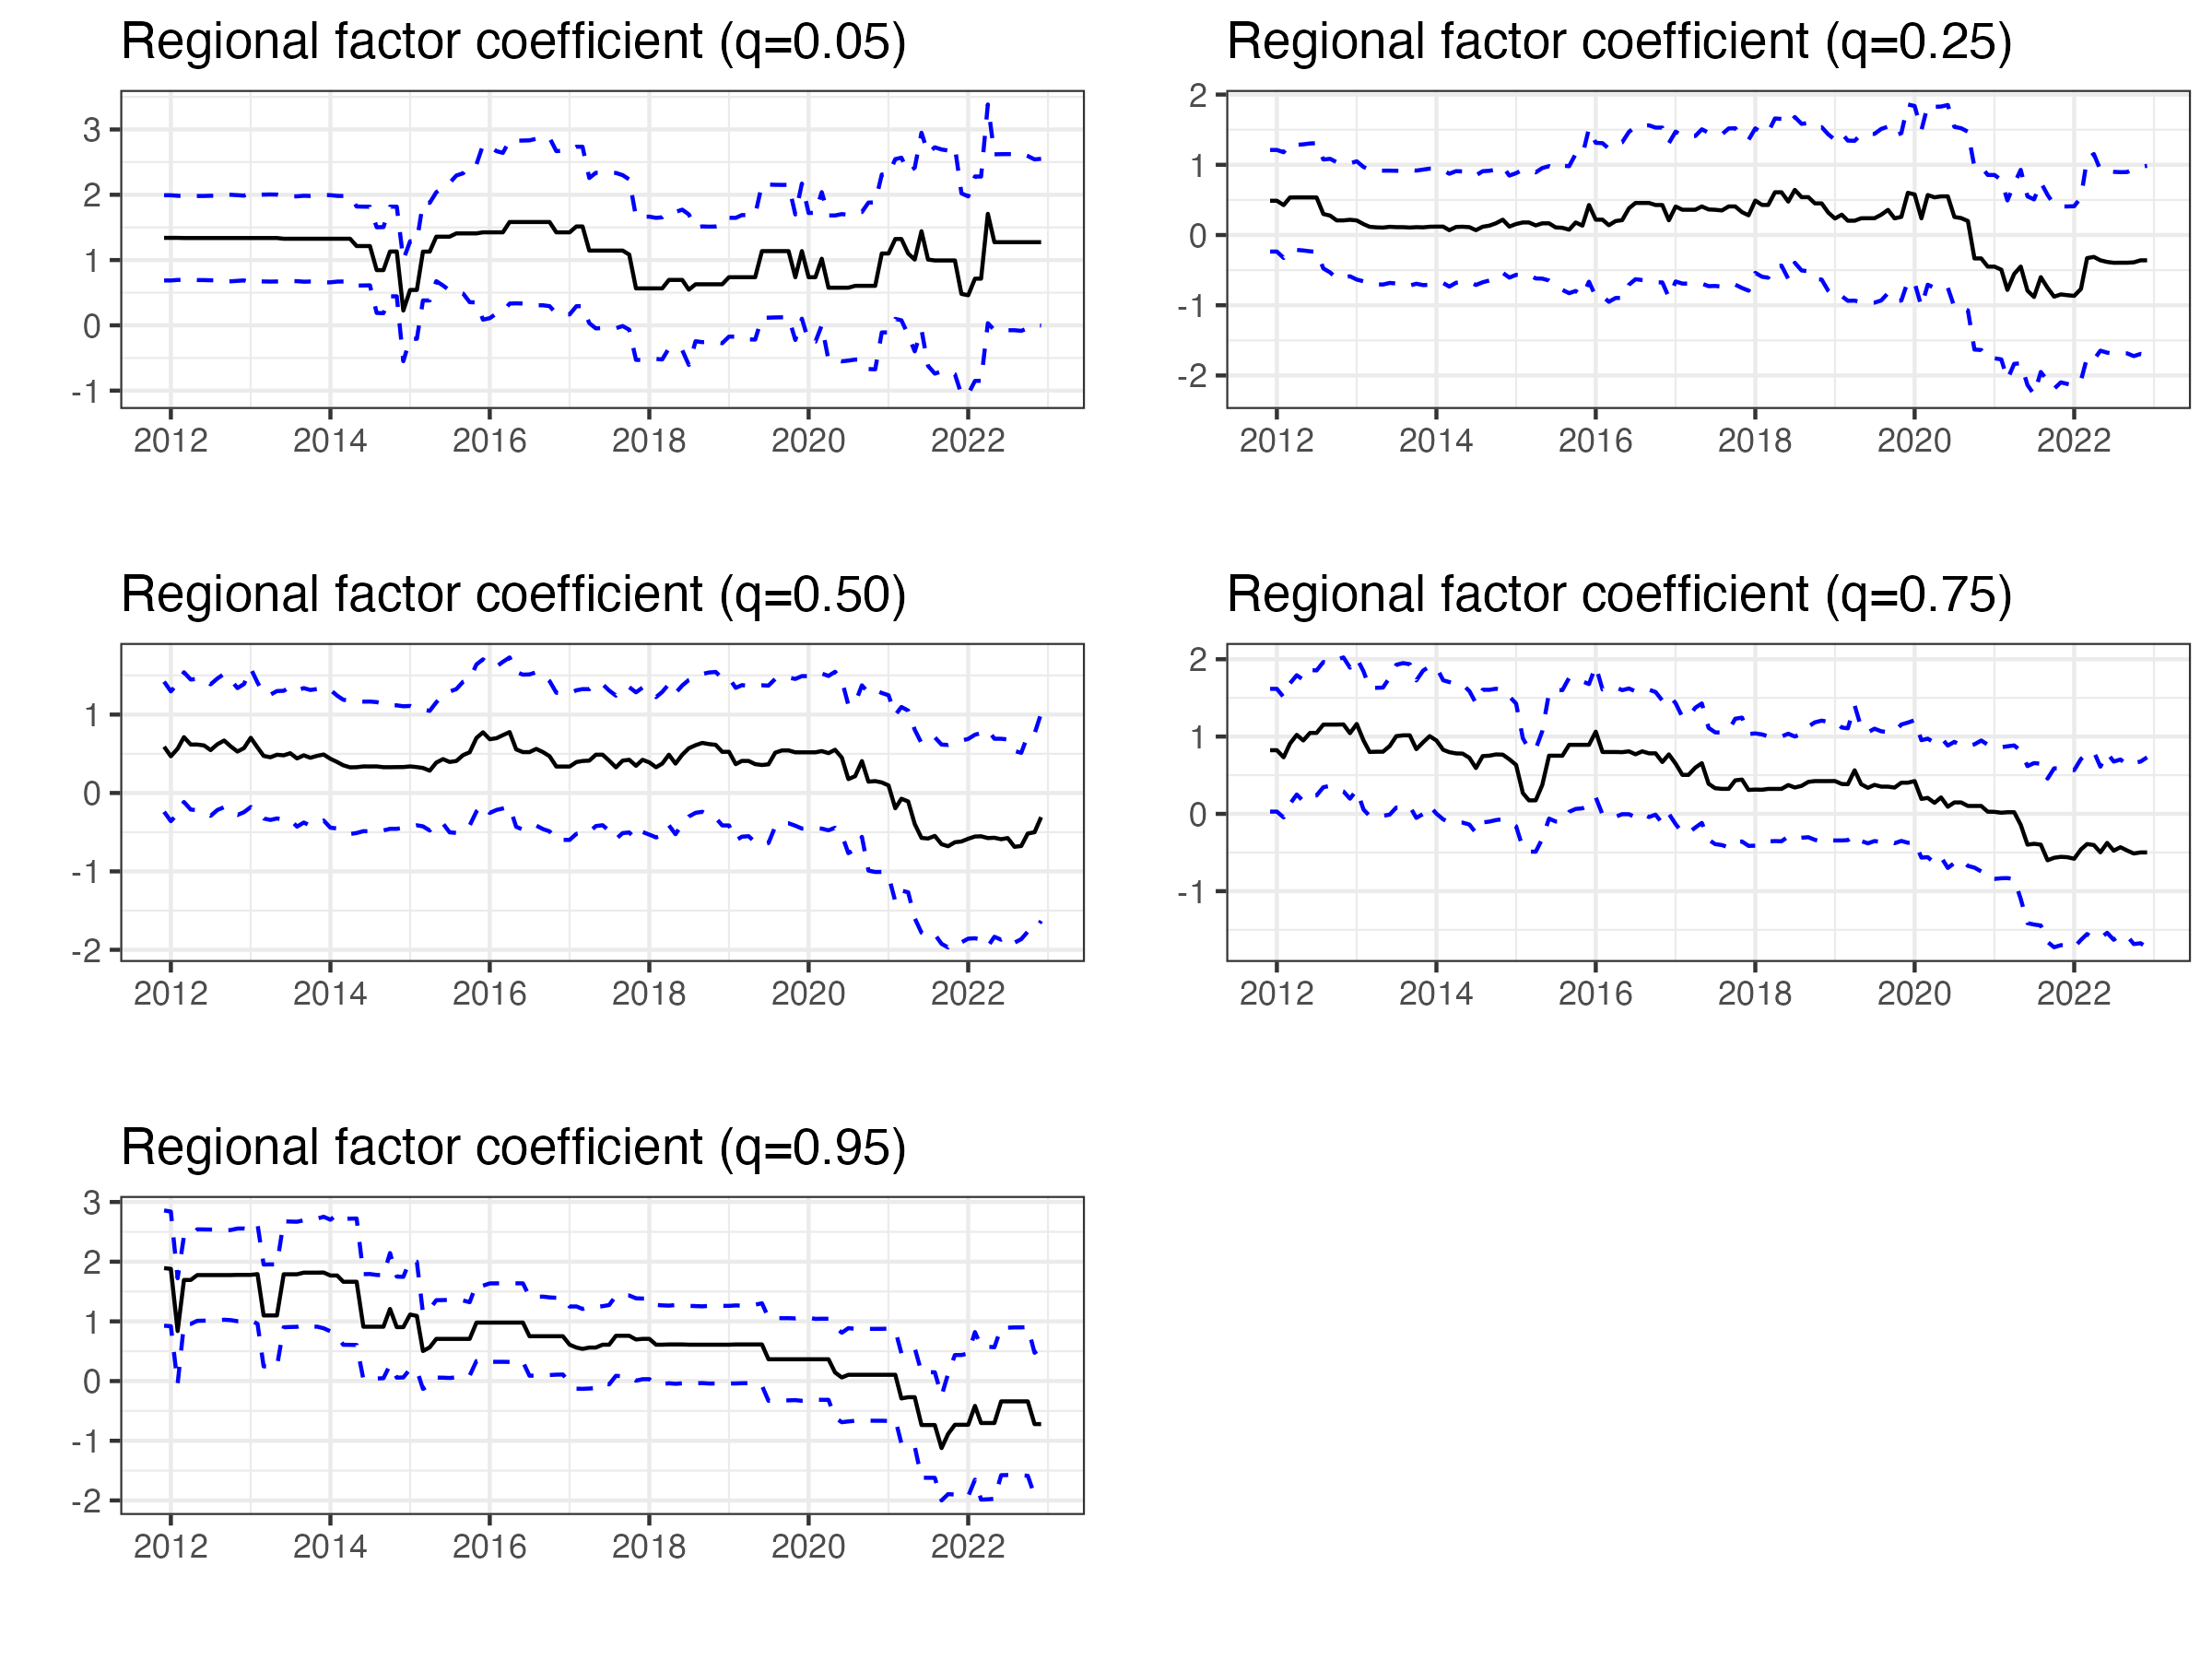}}\\
\subfigure[]{\includegraphics[width=0.30\textwidth]{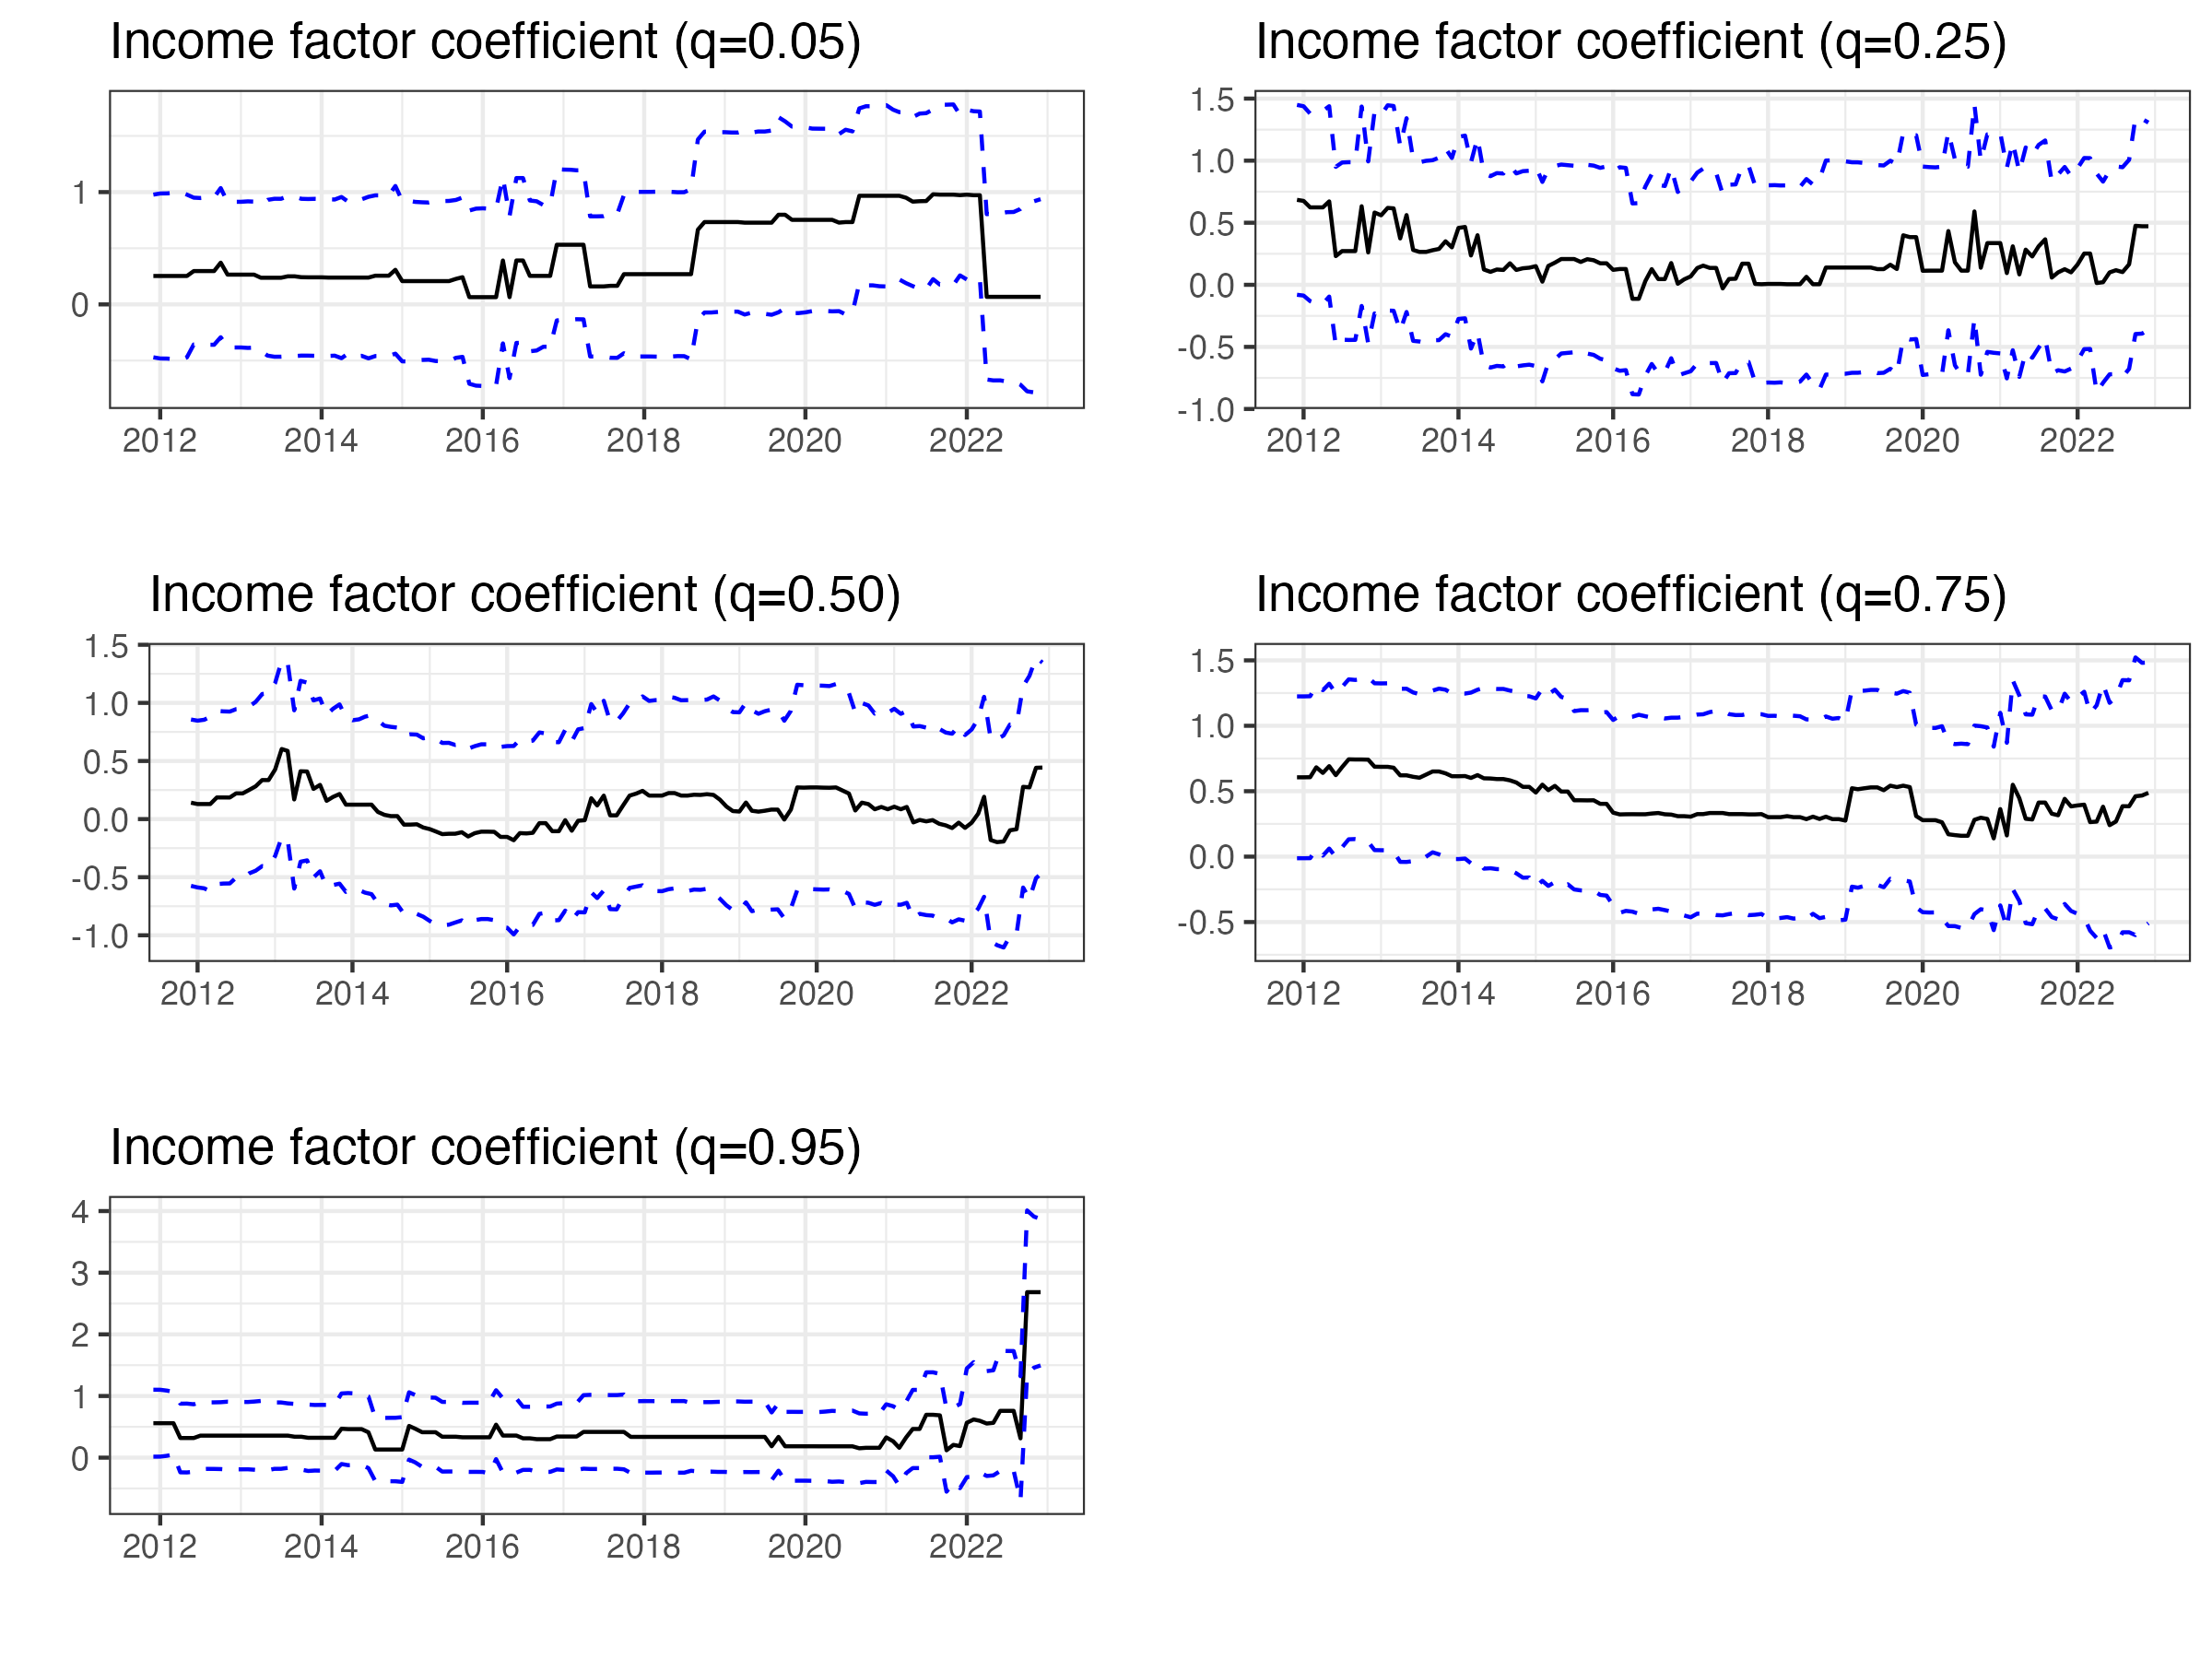}}
\subfigure[]{\includegraphics[width=0.3\textwidth]{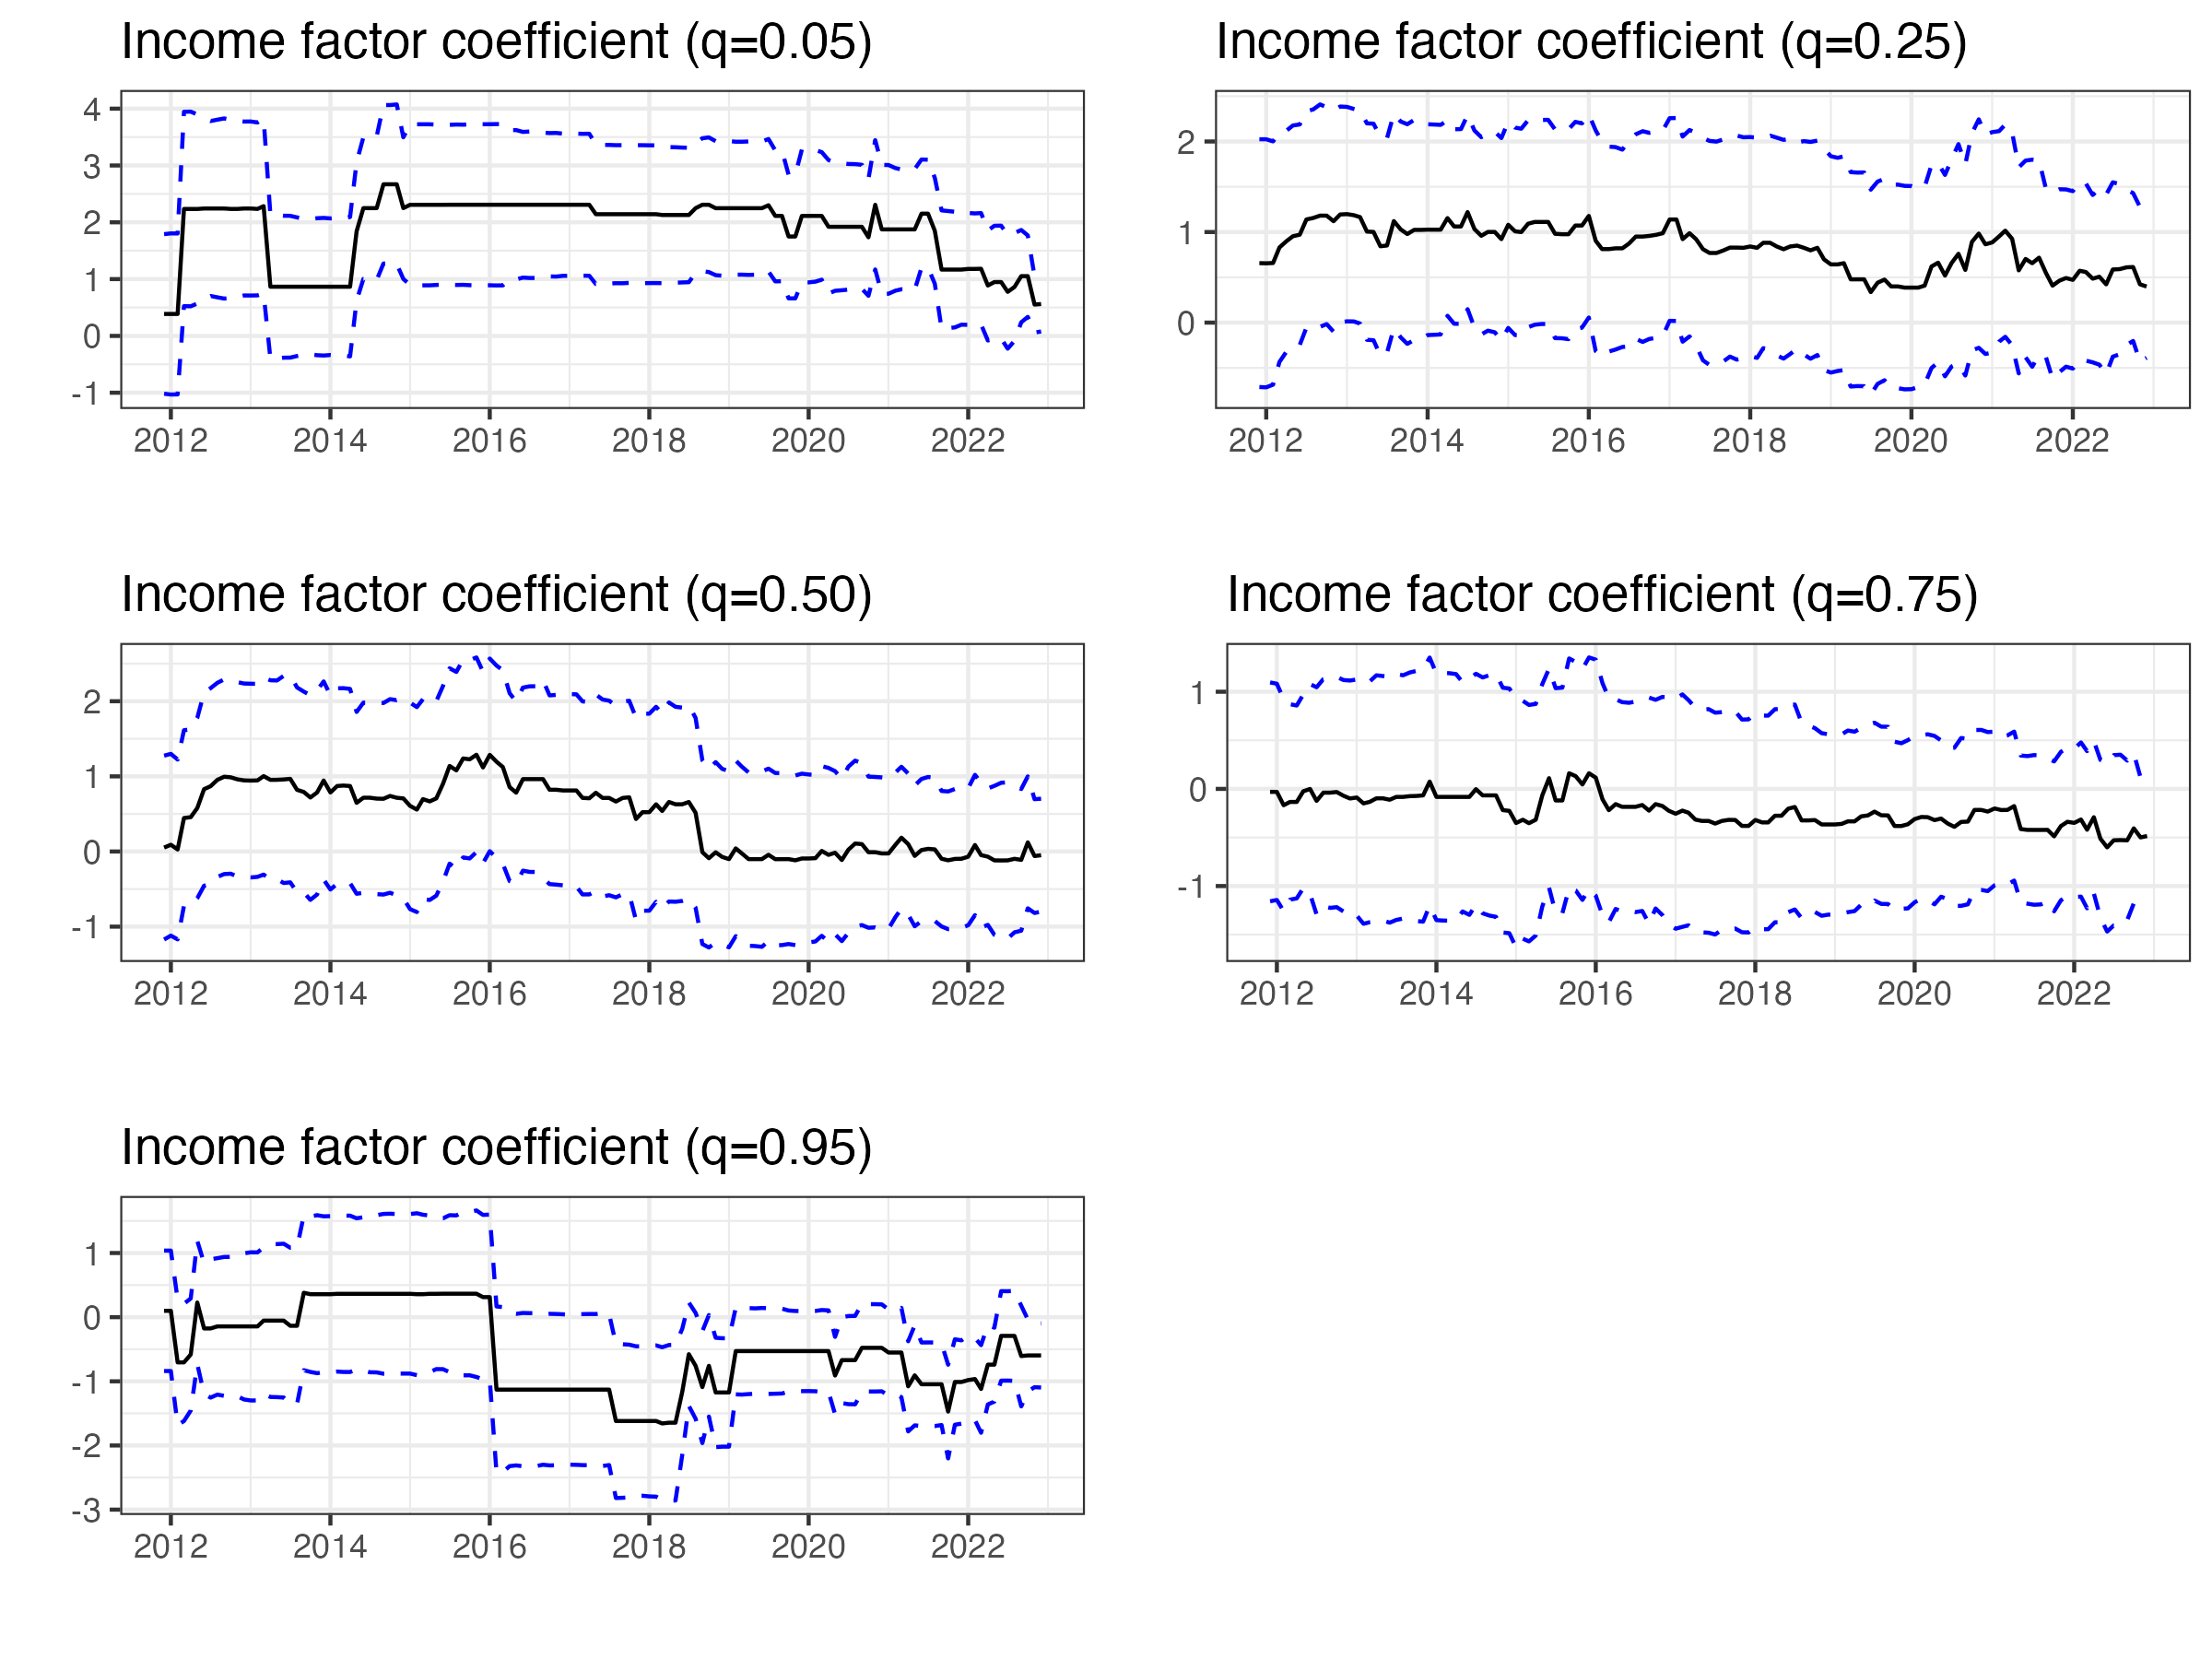}}
\subfigure[]{\includegraphics[width=0.30\textwidth]{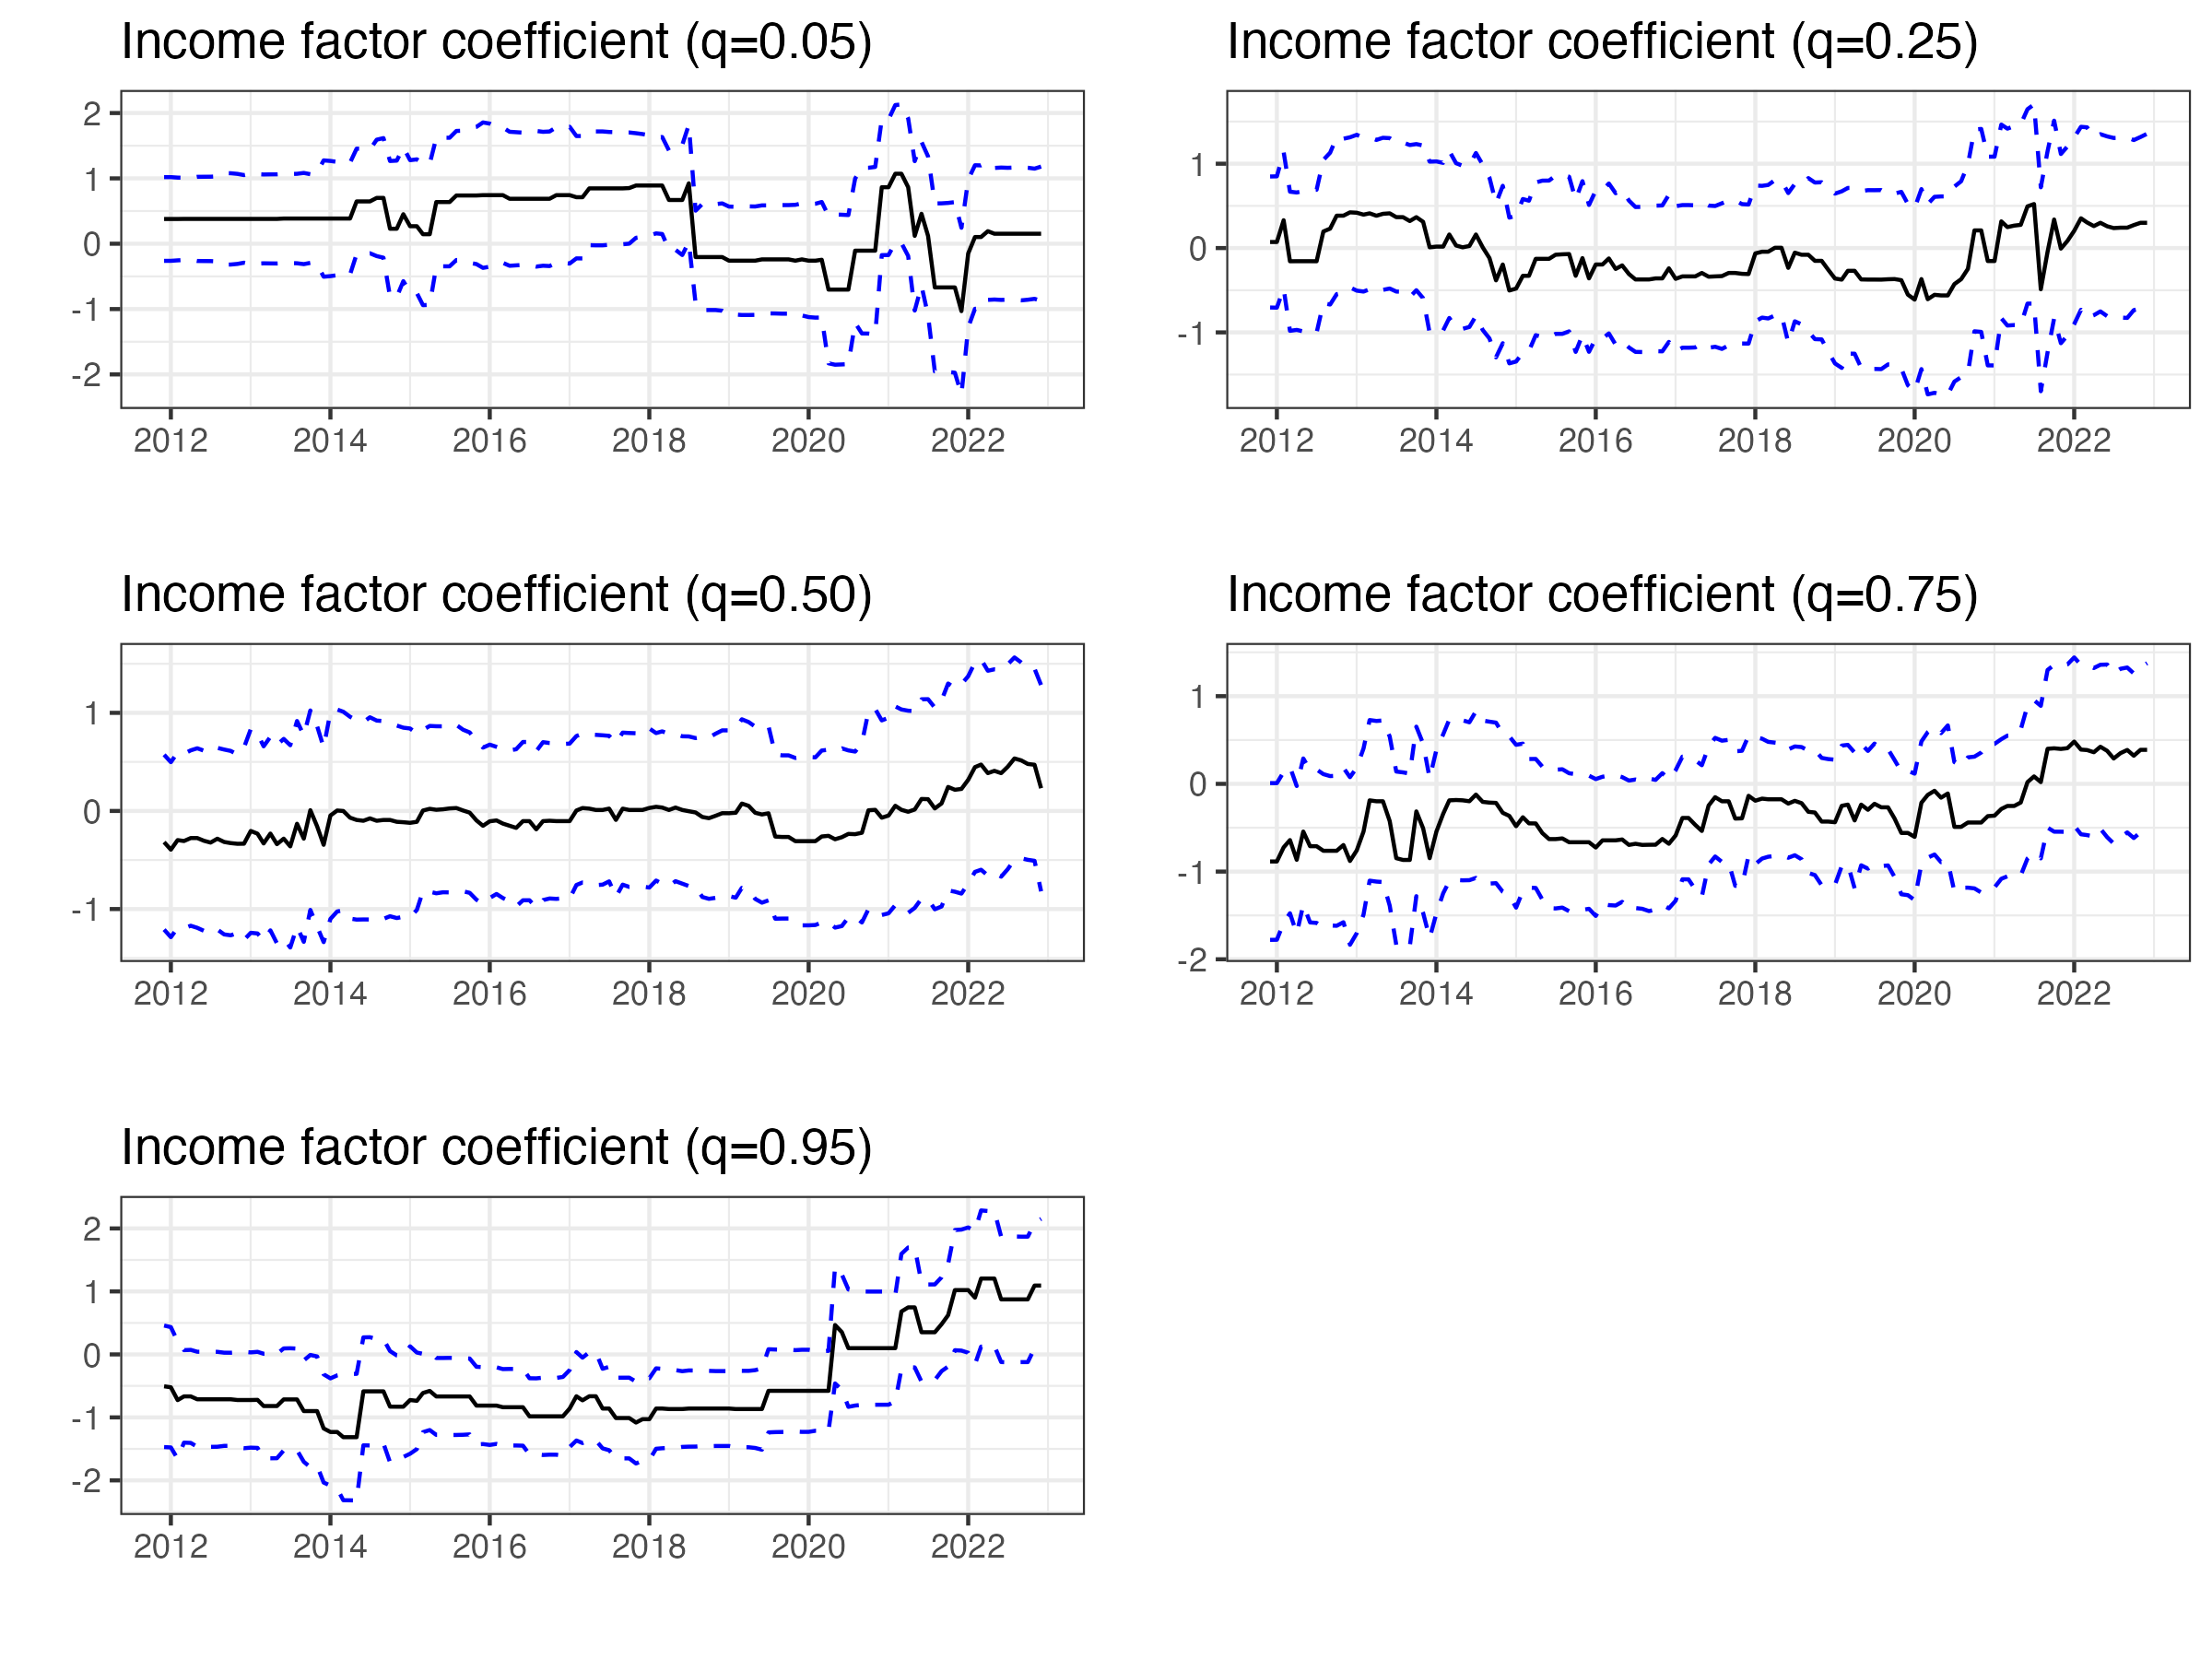}}
\caption{Estimated parameters of FAQR model obtained in the rolling-window: Italy (first column), the US (second column), Mexico (third colmun).}
\label{fig:tv_estimates}
\end{center}
\end{figure}

\newpage

\subsection{Out-of-sample results for restricted FA-QR models.}
\label{appendix:time-varying}

\setcounter{equation}{0}
\setcounter{table}{0}
\setcounter{figure}{0}

\begin{figure}[]
\begin{center}
\includegraphics[width=1\textwidth]{OOS_h_1_QS(0.05).png}
\caption{Ratio of QS for $\tau=0.05$ losses between the FA-QR and AR-QR models.}
\label{fig:Ratio_1}
\end{center}
\end{figure} 

\begin{figure}[]
\begin{center}
\includegraphics[width=1\textwidth]{OOS_h_1_QS(0.50).png}
\caption{Ratio of QS for $\tau=0.50$ losses between the FA-QR and AR-QR models.}
\label{fig:Ratio_2}
\end{center}
\end{figure} 

\begin{figure}[]
\begin{center}
\includegraphics[width=1\textwidth]{OOS_h_1_QS(0.95).png}
\caption{Ratio of QS for $\tau=0.95$ losses between the FA-QR and AR-QR models.}

\label{fig:Ratio_3}
\end{center}
\end{figure}

Figures \ref{fig:Ratio_4} to \ref{fig:Ratio_6} plot the ratios between the CRPS losses for equal, left and right weights, respectively. 

\begin{figure}[]
\begin{center}
\includegraphics[width=1\textwidth]{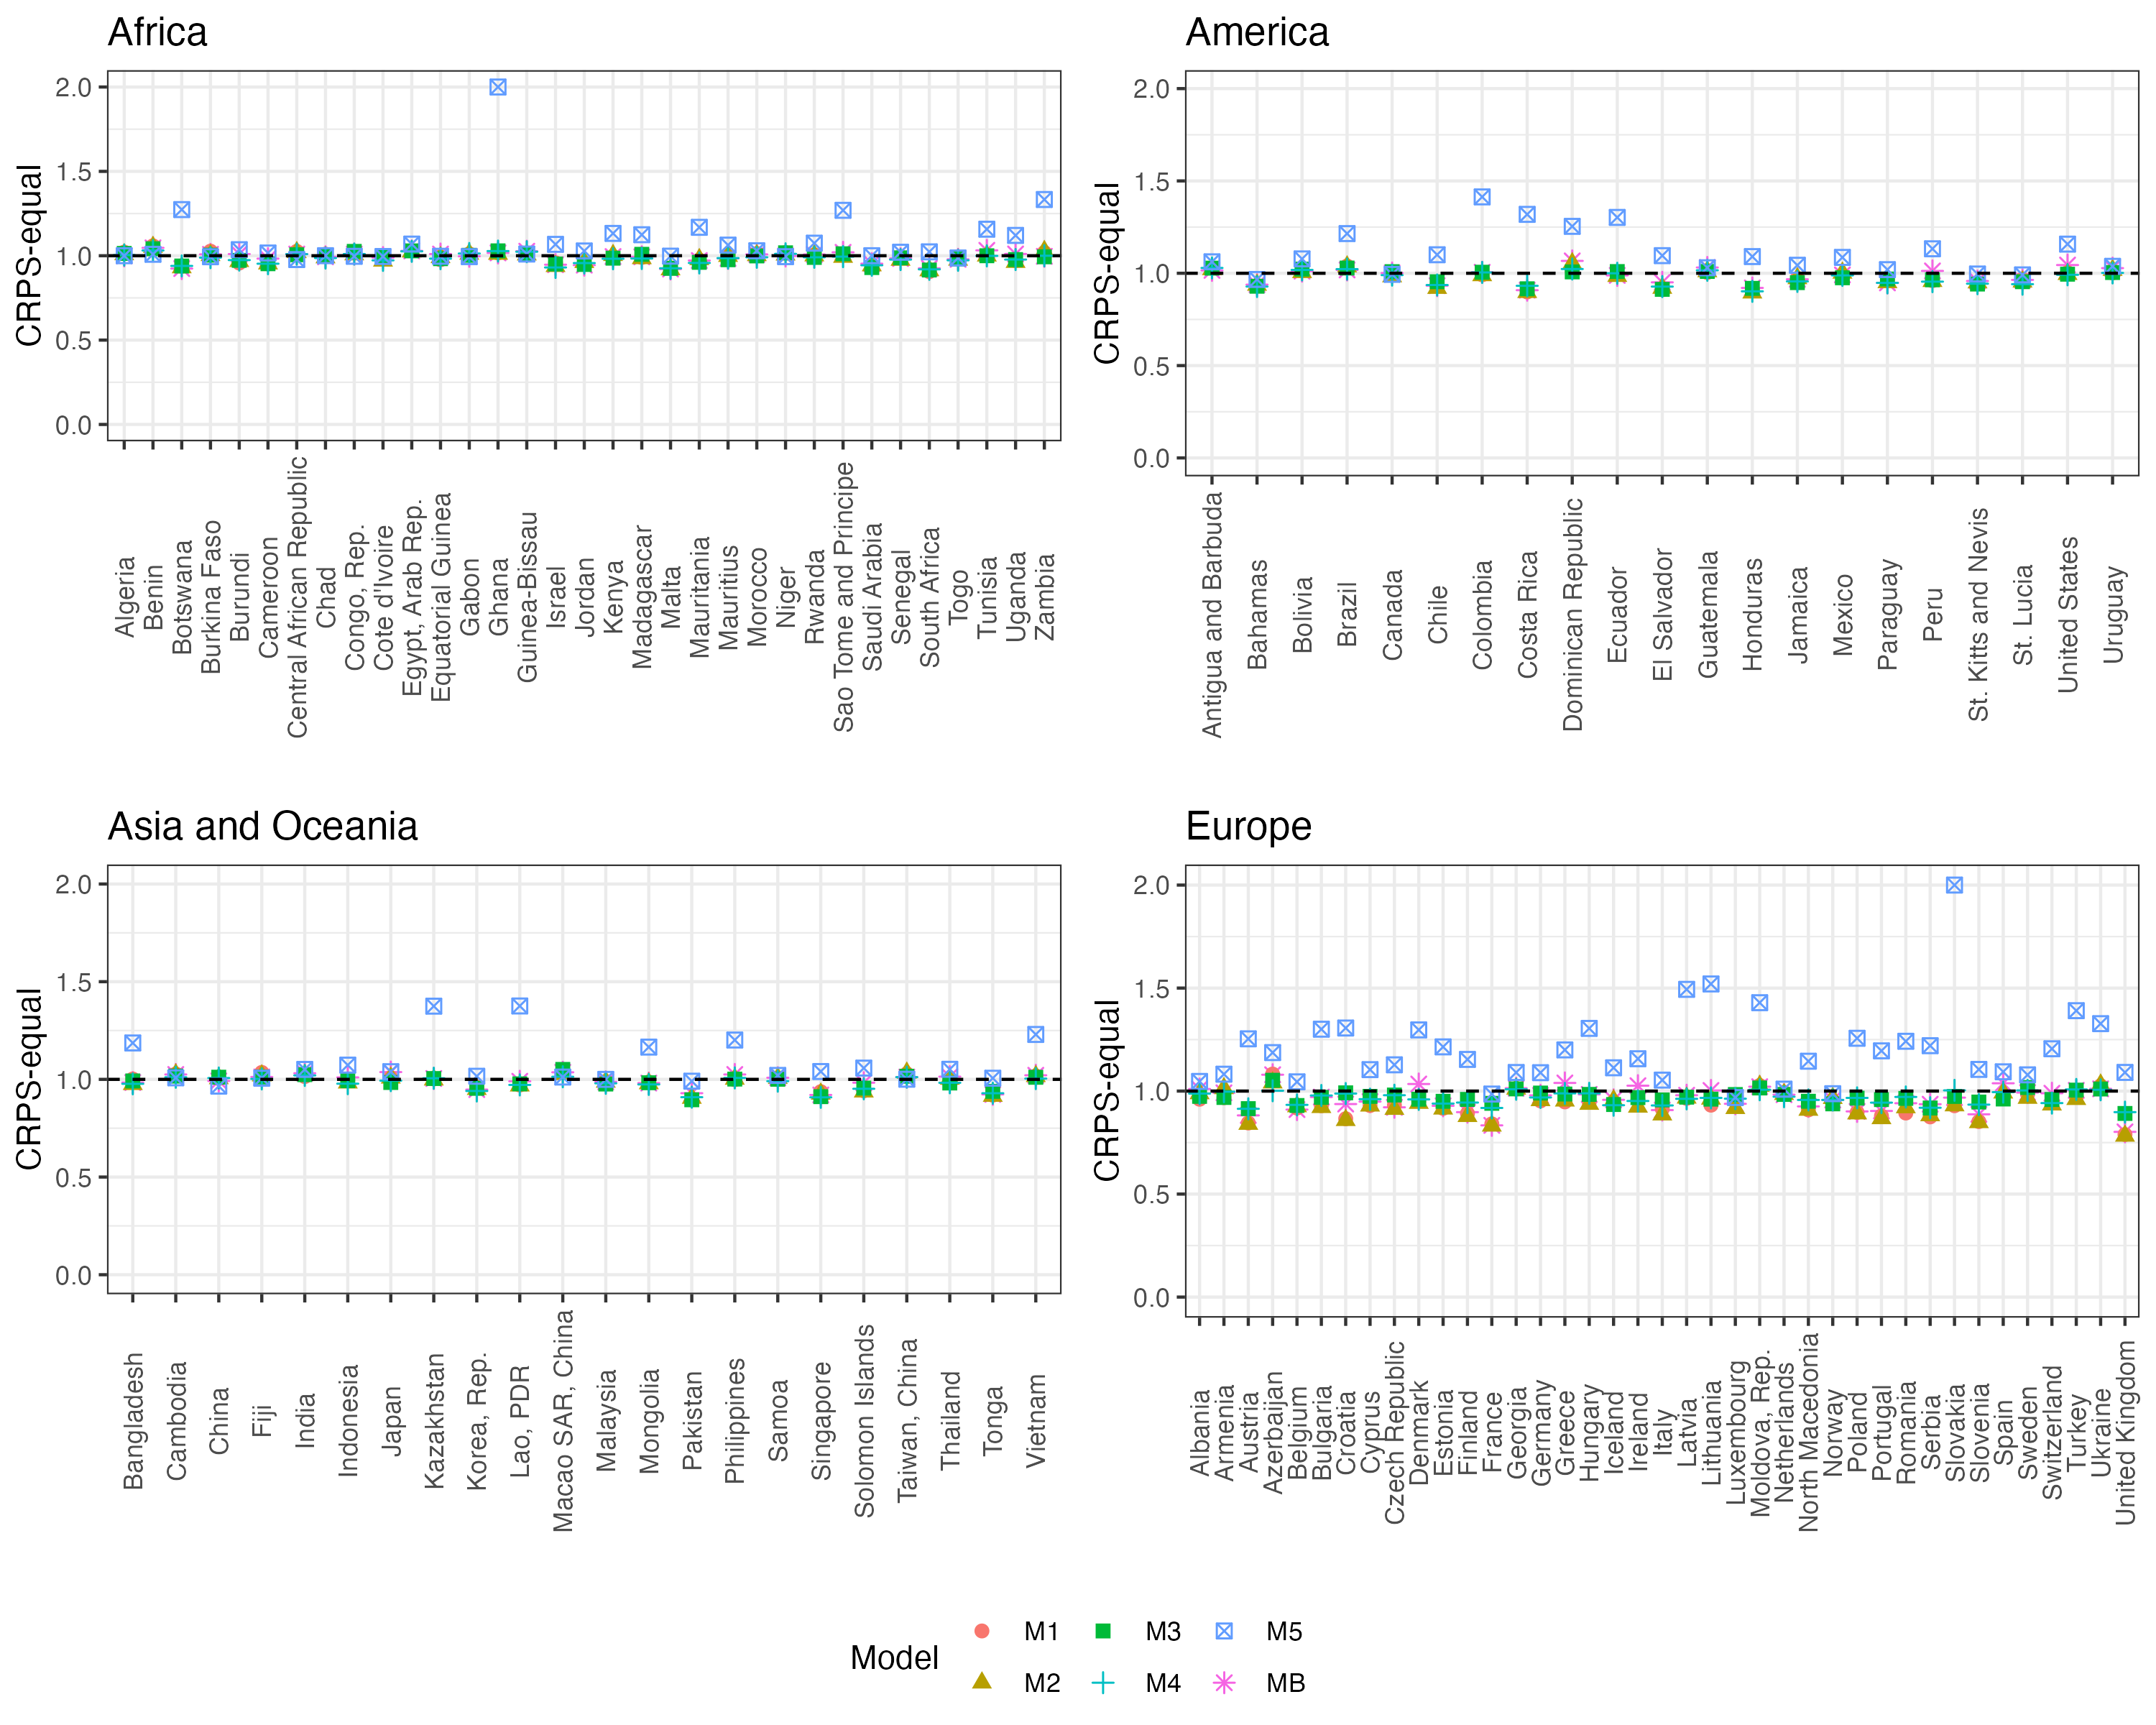}
\caption{Ratio of CRPS loss with equal weights between the FA-QR and AR-QR models.}
\label{fig:Ratio_4}
\end{center}
\end{figure}

\begin{figure}[]
\begin{center}
\includegraphics[width=1\textwidth]{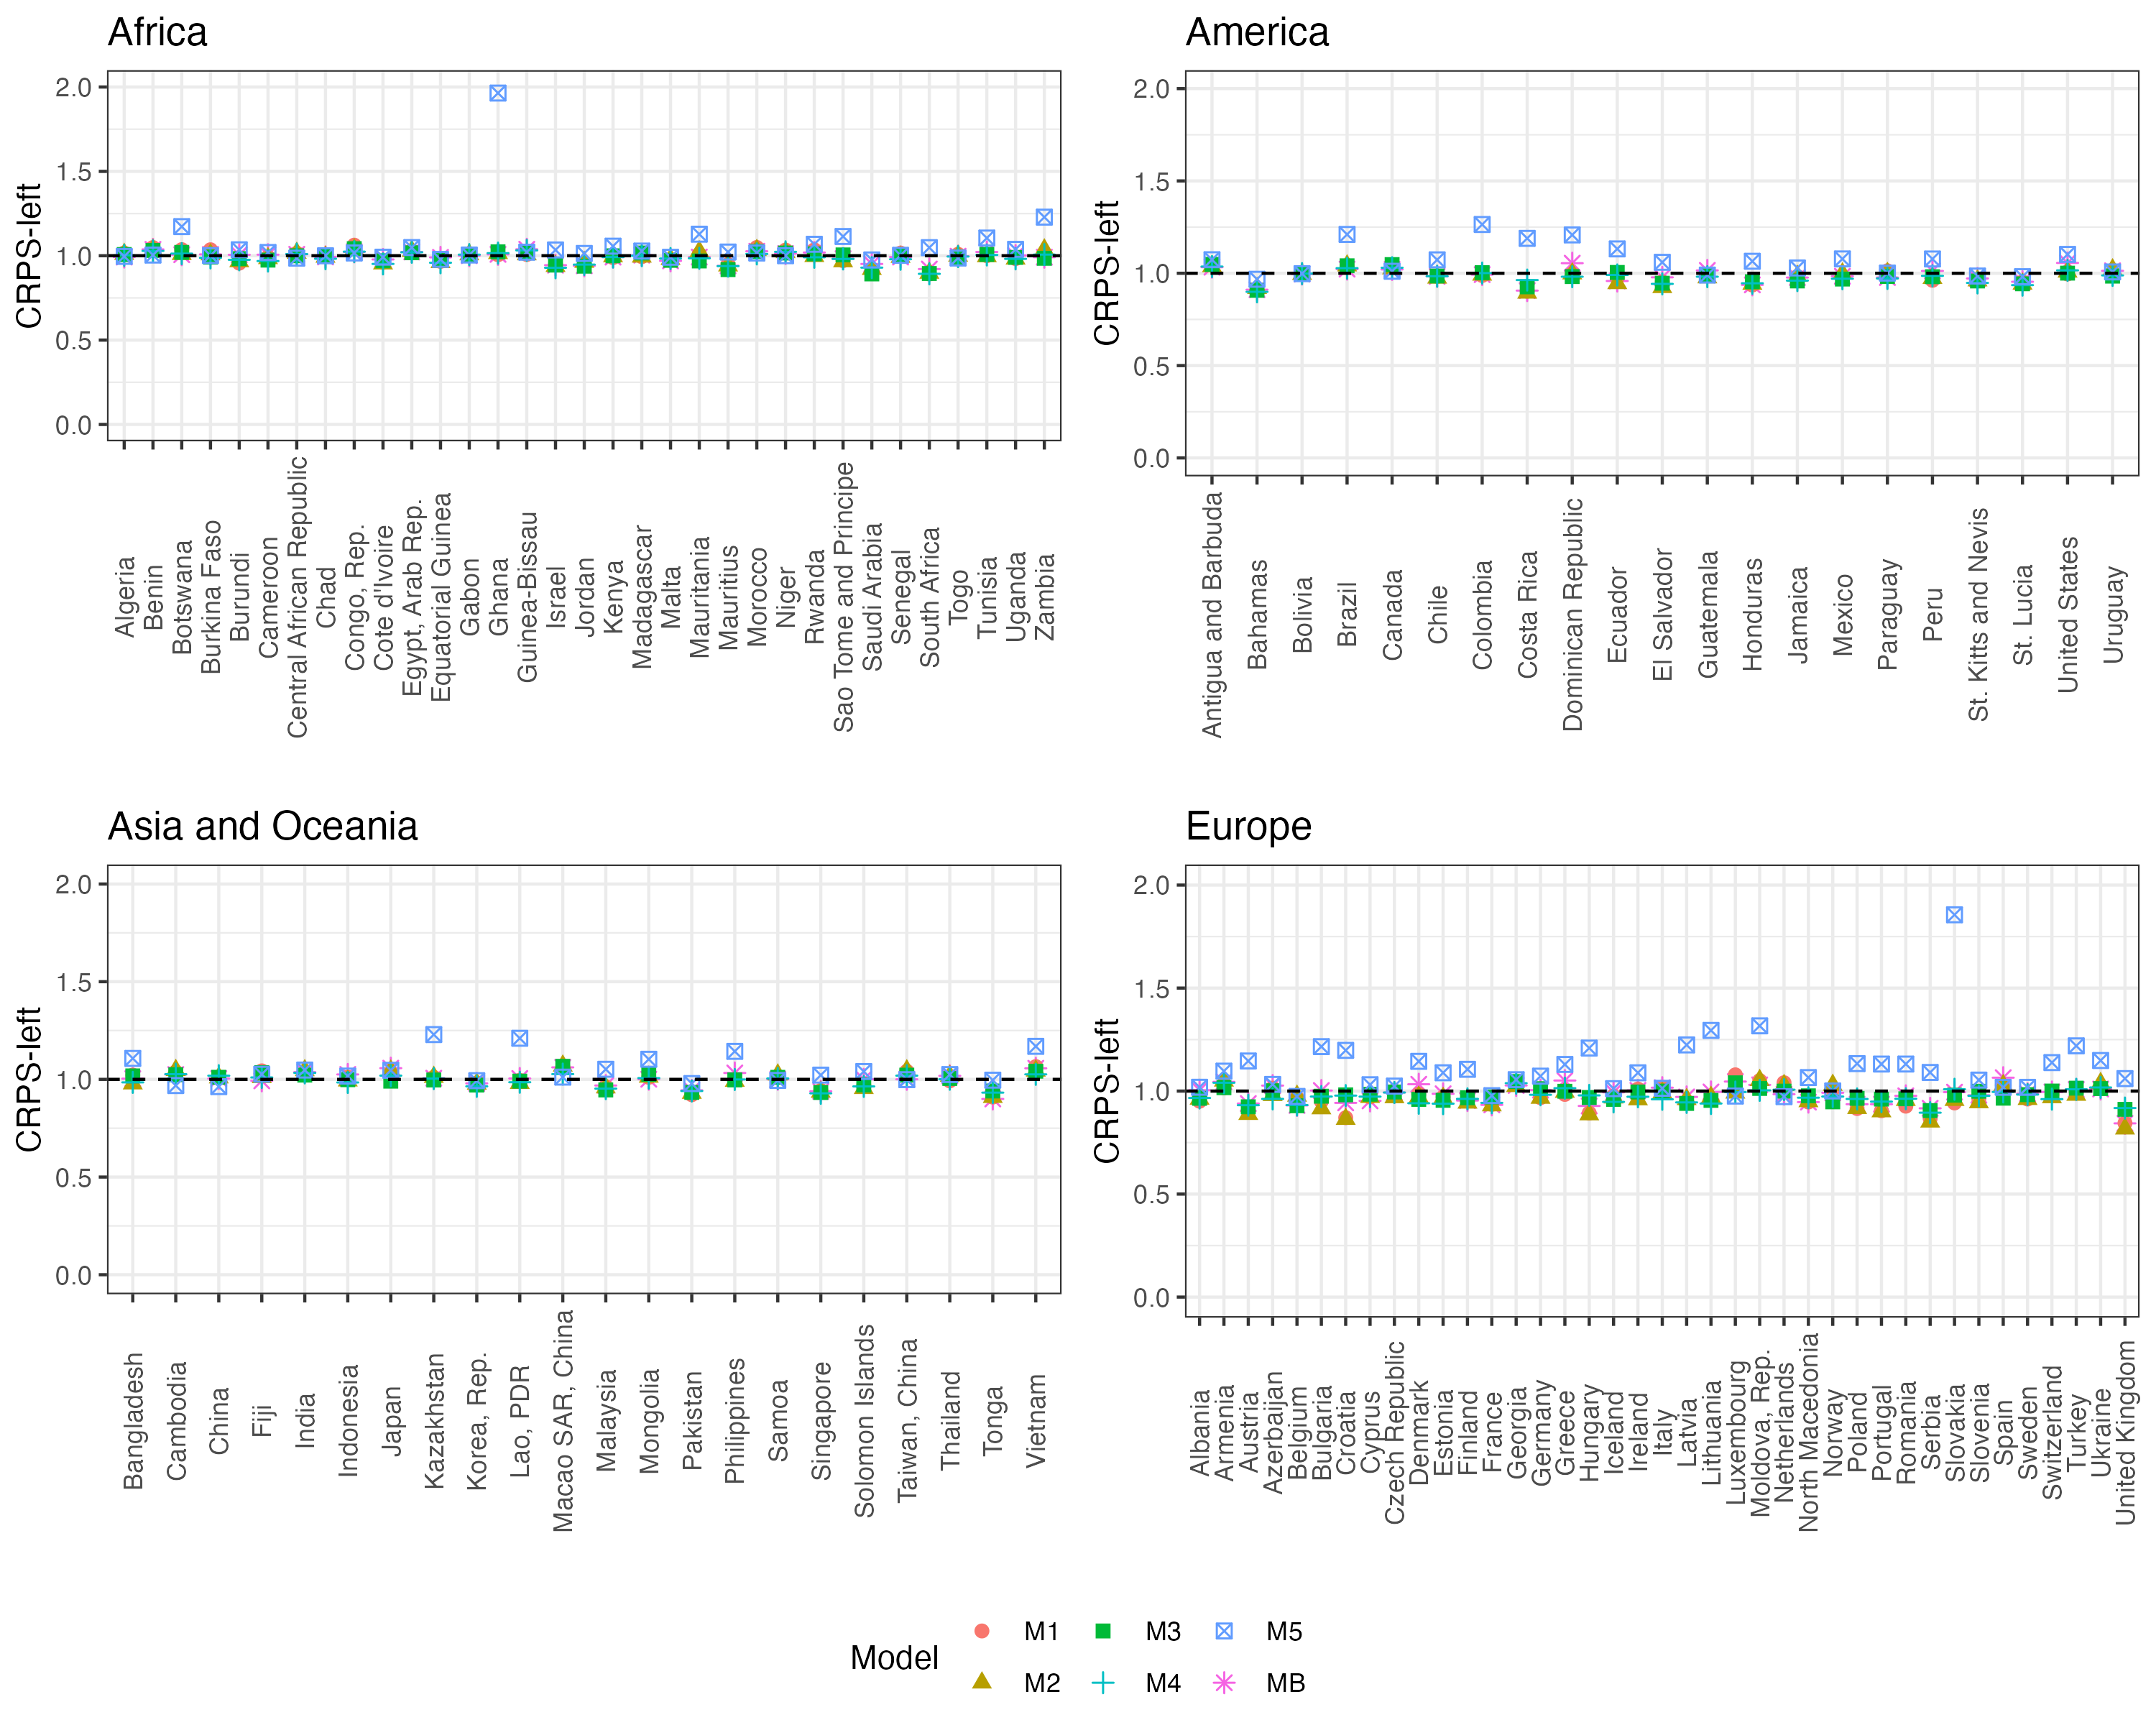}
\caption{Ratio of CRPS loss with left weights between the FA-QR and AR-QR models.}
\label{fig:Ratio_5}
\end{center}
\end{figure}

\begin{figure}[]
\begin{center}
\includegraphics[width=1\textwidth]{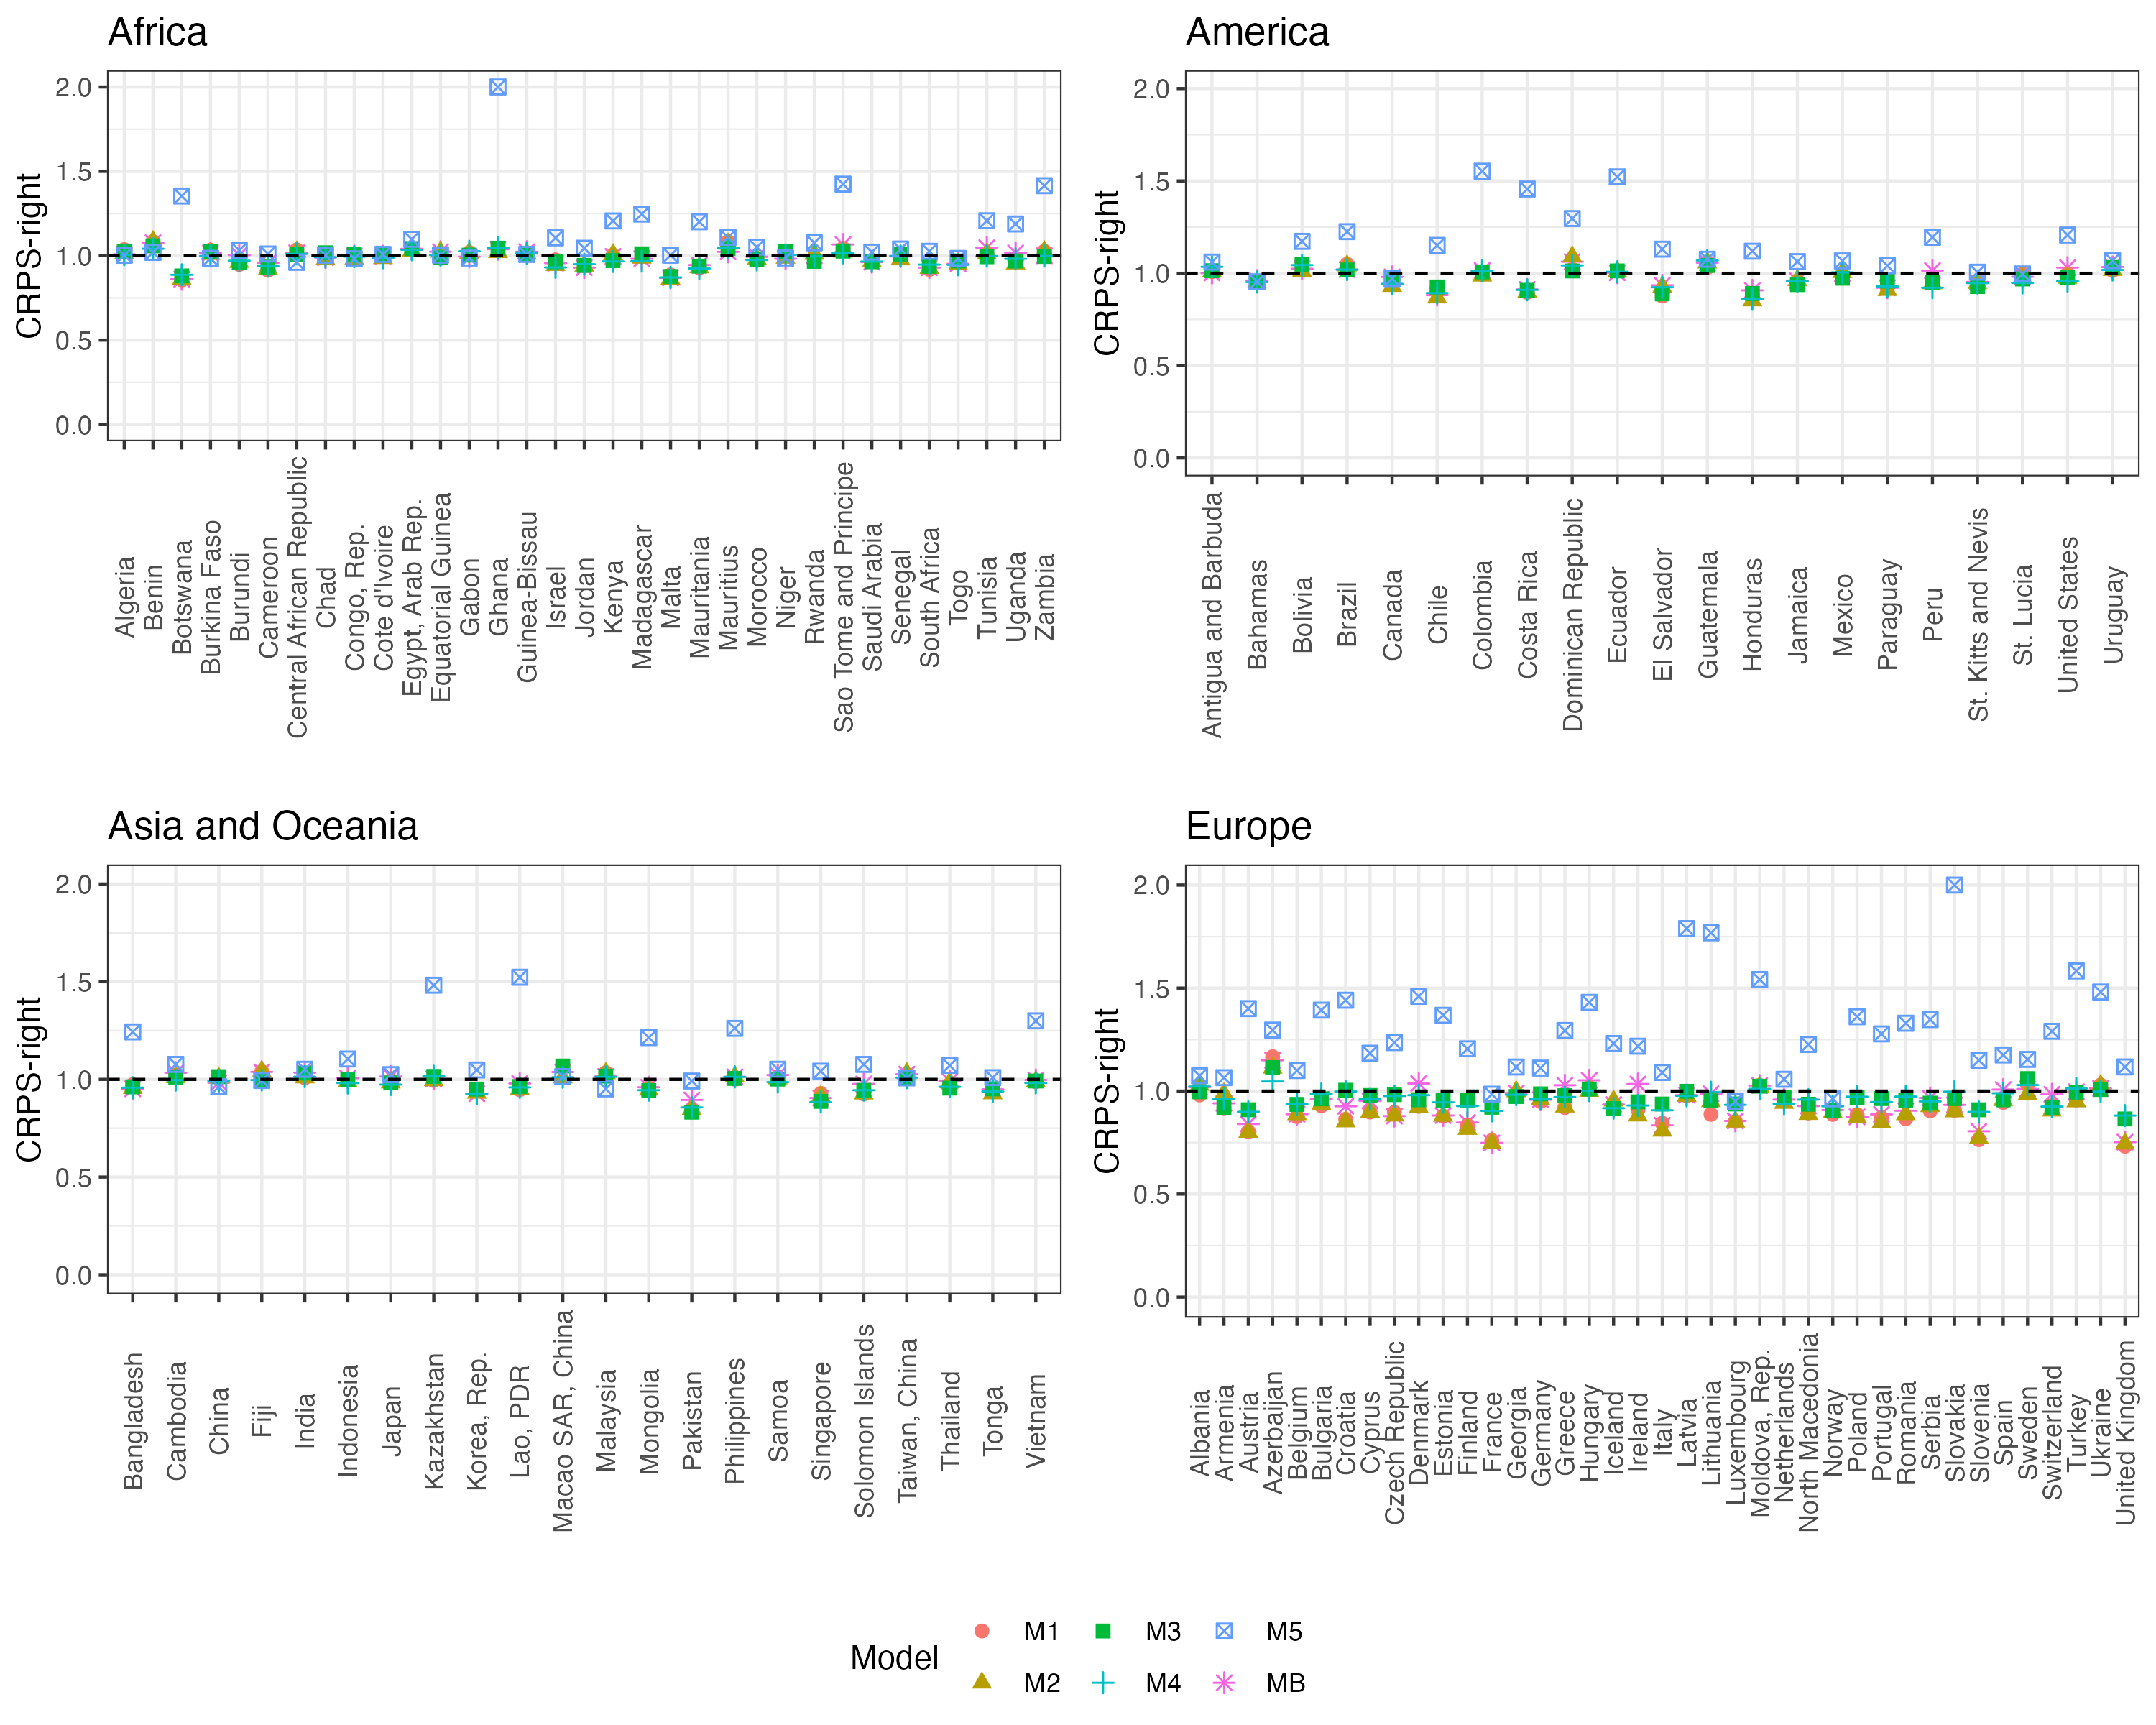}
\caption{Ratio of CRPS loss with right weights between the FA-QR and AR-QR models.}
\label{fig:Ratio_6}
\end{center}
\end{figure}

\section*{References}

Acharya, V., Engle, R., and Richardson, M. (2012). Capital shortfall: a new approach to ranking and regulating systemic risk. \textit{American Economic Review}, 102:59--64.

\end{document}
